# Supplementary material for: QR-LoRA: Efficient and Disentangled Fine-tuning via QR Decomposition for Customized Generation
Source: arXiv:2507.04599 source file (2025-07-24)
Supplement: Supplementary file 1 [file 6_supp.tex]

\twocolumn[
\centering
\Large
\textbf{Appendix of QR-LoRA: Efficient and Disentangled Fine-tuning via QR Decomposition for Customized Generation} \\
(Supplementary Material)
\vspace{+1em}
] %< twocolumn
\appendix

\section{Theoretical Analysis of QR-LoRA Parameter Disentanglement}
% \addcontentsline{toc}{section}{Theoretical Analysis of QR-LoRA Parameter Disentanglement}
\subsection{Minimal Frobenius Norm Property}

\begin{lemma}[Minimal Frobenius Norm Property of QR-LoRA Parameterization]
\label{thm:qr-lora}
Consider a weight matrix \( W \in \mathbb{R}^{m \times n} \) with a low-rank update \( \Delta W = Q \Delta R \), where \( Q \in \mathbb{R}^{m \times r} \) is a column-orthogonal matrix (i.e., \( Q^\top Q = I_r \)), and \( \Delta R \in \mathbb{R}^{r \times n} \) represents trainable parameters. For any rank-\( r \) update \( \Delta W \), the parameterization \( \Delta W = Q \Delta R \) achieves the minimal Frobenius norm if and only if \( Q \) is column-orthogonal, yielding:
\begin{equation}
\| \Delta W \|_F = \| Q \Delta R \|_F = \| \Delta R \|_F,
\end{equation}
with \( \Delta R \) having a unique solution under orthogonal constraints.
\end{lemma}

\begin{proof}
Leveraging the norm-preserving property of orthogonal matrices, for any column-orthogonal \( Q \), we have:
\begin{equation}
\begin{aligned}
\| Q \Delta R \|_F 
&= \sqrt{\text{tr}(\Delta R^\top Q^\top Q \Delta R)} \\
&= \sqrt{\text{tr}(\Delta R^\top \Delta R)} \\
&= \| \Delta R \|_F ,
\end{aligned}
\end{equation}
consequently, the Frobenius norm of the parameterized update \( \Delta W = Q \Delta R \) is equivalent to the norm of \( \Delta R \). 
\end{proof}

This equivalence has profound implications for our framework:
\begin{itemize}
\item \textbf{Minimal Intervention Principle}: The uniqueness of the minimal norm solution reflects the optimal task-specific transformation. For any target weight update \( \Delta W \), we seek its representation in the form of \( Q \Delta R \), where \( Q \) is column-orthogonal. Among multiple solutions satisfying the task objective, the minimal norm solution maximally preserves the model's original generalization capabilities while introducing only necessary task-specific transformations.
\item \textbf{Task-Specific Feature Encoding}: The minimal norm property of \( \Delta R \) prevents overfitting by incorporating only the minimal changes required for the specific task. This principle ensures that \( \Delta R \) exclusively encodes information relevant to the current task, avoiding the incorporation of general features shared across different tasks.
\end{itemize}

\subsection{Gradient Update Decoupling Analysis}

\begin{theorem}[Statistical Independence of Orthogonal Projections]
\label{thm:orthogonal-projections}
In a Hilbert space with orthogonal basis, projections along different feature directions are statistically independent. Specifically, for any two orthogonal directions $v_i$ and $v_j$ ($v_i^\top v_j = 0$), the projections of a random vector $x$ onto these directions, denoted as $P_i(x)$ and $P_j(x)$ respectively, are statistically uncorrelated:
\begin{equation}
E[P_i(x)P_j(x)] = 0,
\end{equation}
where $E[\cdot]$ denotes the expectation operator.
\end{theorem}

In the context of Hilbert spaces with orthogonal bases, projections along different feature directions exhibit statistical independence. This fundamental property plays a crucial role in our QR-LoRA framework, where the $Q$ matrix defines a set of orthogonal basis vectors, and the $\Delta R$ matrix represents coordinates in this orthogonal basis system. The gradient update mechanism in our framework demonstrates how this orthogonality naturally leads to feature disentanglement.
For a loss function \( \mathcal{L}(W) \) with the parameterization \( W = W_{\text{comp}} + Q(R + \Delta R) \), the gradient update mechanism exhibits the following key property:

The gradient of the loss with respect to \( \Delta R \) is given by:
\begin{equation}
\frac{\partial \mathcal{L}}{\partial \Delta R} 
= \frac{\partial\mathcal{L}}{\partial W}\cdot\frac{\partial W}{\partial\Delta R}
= Q^\top \frac{\partial \mathcal{L}}{\partial W}.
\label{eq:gradient}
\end{equation}

Given the column orthogonality of \( Q \) (\( Q^\top Q = I \)), this gradient formulation reveals that \( \partial \mathcal{L}/\partial \Delta R \) is an orthogonal projection of \( \partial \mathcal{L}/\partial W \) onto the column space of \( Q \). This projection mechanism is particularly significant when training for different tasks (\eg, style or content adaptation), as these tasks inherently optimize distinct visual attributes. The orthogonality of their gradient directions in the high-dimensional space is preserved and enhanced through the $Q$ matrix projection, causing different $\Delta R$ matrices to evolve along approximately orthogonal trajectories during training.

To provide a comprehensive understanding of QR-LoRA's theoretical advantages, we further analyze its forward pass and gradient computation mechanisms in comparison with existing methods. Table~\ref{tab:method-comparison} presents a detailed comparison of the forward pass and gradient computation between QR-LoRA and other representative approaches.

\begin{table*}[h]
\caption{\textbf{Summary of forward pass and gradient computation in different methods.} This comparison highlights QR-LoRA's unique orthogonal projection-based gradient update mechanism, which naturally leads to more effective feature disentanglement compared to traditional approaches.}
% \vspace{-3.5mm}
\centering
\label{tab:method-comparison}
\resizebox{0.8\linewidth}{!}{
% \scriptsize 
\begin{tabular}{cccc} \toprule
\multicolumn{1}{l}{} & \multicolumn{1}{c}{LoRA \cite{hu2021lora}} & \multicolumn{1}{c}{Ortha \cite{po2024orthogonal}} & \multicolumn{1}{c}{QR-LoRA} \\ \midrule
\multirow{3}{*}{\begin{tabular}[c]{@{}l@{}}Forward\end{tabular}} 
& $Y\!\!=\!\!X(W\!\!+\!\!BA)$ & $Y\!\!=\!\!X(W\!\!+\!\!BA)$ & $Y=XW; W\!=\!U\Sigma V^\top$ \\
& $A\!\!\sim \!\! \mathcal{N}\!(\!0,\!\sigma^2\!) \!\!\in\!\! \mathbb{R}^{r\times n}$ & $A\!\!\sim \!\! \mathcal{N}\!(\!0,\!\sigma^2\!) \!\!\in\!\! \mathbb{R}^{r\times n}$ & $W_{core}^\top\!=\!V_{[:r,:]}\Sigma_{[:r]} U_{[:,:r]}^\top\!=\!QR$ \\
& $B\!=\!0\!\in\! \mathbb{R}^{m\times r}$ & $B\!\!\sim \!\! \mathcal{N}\!(\!0,\!\sigma^2\!) \!\!\in\!\! \mathbb{R}^{m\times r}$ &  $W\!=\!W_{comp}+(Q(R+\Delta R))^\top$\\ \midrule
\multirow{2}{*}{\begin{tabular}[c]{@{}l@{}}Gradient\end{tabular}} 
& $\frac{\partial\mathcal{L}}{\partial A} \!\!=\!\! B^\top \! \!\frac{\partial\mathcal{L}}{\partial W} \!\!\Rightarrow \!\textbf{ 0}$ & frozen $B$, train $A$ & $Q\!\!\in\!\! \mathbb{R}^{n\times r}\!,\!R\!\!\in\!\! \mathbb{R}^{r\times m}$; train $\Delta R$ \\
& $\frac{\partial\mathcal{L}}{\partial B}\!\! = \!\!\frac{\partial\mathcal{L}}{\partial W}\! A^\top \!\!\Rightarrow \!\textbf{ Random}$ & $\frac{\partial\mathcal{L}}{\partial A} \!\!= \!\!B^\top\!\! \frac{\partial\mathcal{L}}{\partial W} \!\!\Rightarrow \!\textbf{Random} $ & $\frac{\partial\mathcal{L}}{\partial \Delta R}\!\! =\!\! Q^\top \!\!\frac{\partial\mathcal{L}}{\partial W} \!\!\Rightarrow \!\textbf{Primary}$ \\ 
\bottomrule
\end{tabular}
}
% \vspace{-3.5mm}
\end{table*}
As shown in Table~\ref{tab:method-comparison}, QR-LoRA fundamentally differs from previous approaches in both its forward pass computation and gradient update mechanism. While traditional LoRA \cite{hu2021lora} and Ortha \cite{po2024orthogonal} rely on random initialization and direct parameter updates, our method leverages orthogonal decomposition to achieve more principled and effective parameter updates.

\subsection{Theoretical Interpretation of Experimental Observations}

\begin{itemize}
\item \textbf{Stability of $Q$}: The stability of \( Q \) matrices across different tasks stems from their construction through SVD-based QR decomposition, where their directions are primarily determined by the underlying data distribution, leading to consistently high similarities.
\item \textbf{Independence of $\Delta R$}: The orthogonal projection property ensures that \( \Delta R \) matrices exclusively capture task-specific information, resulting in significant variations that reflect the unique characteristics of different tasks.
\end{itemize}

\begin{figure}[t]
    \centering
    \includegraphics[width=\linewidth]{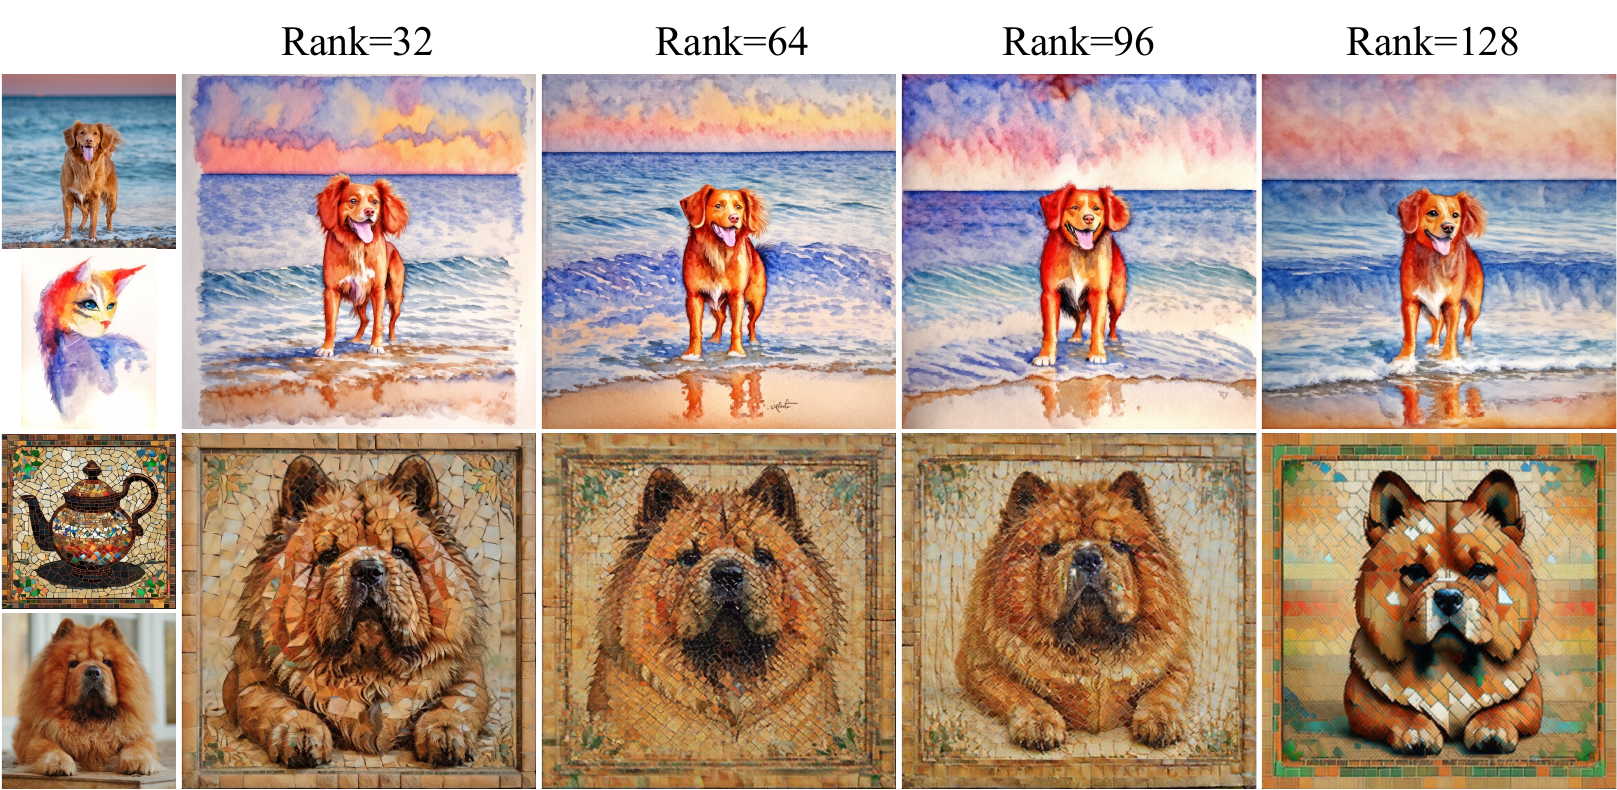}
    \caption{\textbf{Rank sensitivity analysis.} Our method maintains stable performance across different rank settings, demonstrating its robustness to this hyperparameter choice.}
    \label{fig:rank_ablation}
\end{figure}

\section{Additional Implementation Details} 

\subsection{Implementation Details of Compared Methods.}
In our comprehensive evaluation, we implement ZipLoRA based on an unofficial implementation\footnote{https://github.com/mkshing/ziplora-pytorch}, configuring it with rank $r=64$ and learning rate $5e\text{-}5$. For StyleAligned and B-LoRA, we adopt their respective default configurations from the original papers. Additionally, we employ the standard DreamBooth-LoRA implementation for experiments on SD3 and FLUX.1-dev models, maintaining consistent hyperparameters ($r=64$, lr=$1e\text{-}4$) across all comparisons to ensure fairness.

\textbf{Model-specific Training Configurations.}
Across all backbone models, we exclusively inject QR-LoRA modules into the main generative networks (\eg, UNet, MM-DiT) while keeping the text encoders frozen during training. For different backbone models, we inject QR-LoRA modules into specific layers as shown in Table~\ref{tab:target-layers}:
\begin{itemize}
\item \textbf{SDXL}: We inject our QR-LoRA modules into the self-attention layers of UNet only, focusing on the core architecture components. For inference, we use 50 denoising steps while keeping other parameters at their default values.
\item \textbf{SD3}: Following the model architecture, we apply our method to both standard attention blocks and additional projection layers unique to SD3. During inference, we employ 28 denoising steps with default configurations for other parameters.
\item \textbf{FLUX.1-dev}: We extend the injection to include both attention mechanisms and feedforward networks, covering the expanded architecture of FLUX.1-dev. Similar to SD3, we use 28 denoising steps for inference while maintaining default settings for other parameters.
\end{itemize}

\begin{table}[]
\centering
% \caption{Model Architecture Components Comparison}
\caption{\textbf{Injection layer types of QR-LoRA across different backbone models.} This table details the specific architectural components where our QR-LoRA modules are injected during training across different foundation models (SDXL, SD3, and FLUX.1-dev), demonstrating the practical implementation of our method's disentangled fine-tuning approach.}
\label{tab:target-layers}
\begin{tabular}{p{1.8cm}p{2.2cm}p{3.2cm}@{}}
\toprule
\textbf{SDXL} & \textbf{SD3} & \textbf{FLUX.1-dev} \\
\midrule
to\_k         & attn.to\_k     & attn.to\_k        \\
to\_q         & attn.to\_q     & attn.to\_q        \\
to\_v         & attn.to\_v     & attn.to\_v        \\
to\_out.0     & attn.to\_out.0 & attn.to\_out.0    \\
\cmidrule(lr){2-3} 
              & attn.add\_k\_proj & attn.add\_k\_proj \\
              & attn.add\_q\_proj & attn.add\_q\_proj \\
              & attn.add\_v\_proj & attn.add\_v\_proj \\
              & attn.to\_add\_out & attn.to\_add\_out \\
\cmidrule(lr){3-3}
              &               & ff.net.0.proj    \\
              &               & ff.net.2         \\
              &               & ff\_context.net.0.proj \\
              &               & ff\_context.net.2 \\
\bottomrule
\end{tabular}
\end{table}

\section{Additional Analysis Details and Results} 

\subsection{Experimental Setup for Matrix Similarity Analysis}
To comprehensively evaluate the feature disentanglement capabilities of our QR-LoRA framework, we conduct extensive experiments using 27 randomly selected image pairs (sample index from 0-26), as visualized in Figure~\ref{fig:appendix-fig2}. For each image pair, we analyze three different training strategies: (1) a QR decomposition variant where both $Q$ and $R$ matrices are directly fine-tuned, (2) a $\Delta R$-only update strategy, and (3) vanilla LoRA with $A$ and $B$ matrices. The cosine similarities between corresponding matrices across different training instances are computed and recorded in Table~\ref{tab:matrix-similarity}, with their distributions visualized in Figure~\ref{fig:matrix-comparsion} of the main text. This experimental design allows us to analyze the inherent properties of different matrices and their roles in feature representation.

\subsection{Cross-Model Analysis of Matrix Properties}
We extend our analysis across three state-of-the-art text-to-image models: SDXL, SD3, and FLUX.1-dev, to validate the model-agnostic nature of our approach. As shown in Figure~\ref{fig:appendix-fig3-sdxl-multi}, Figure~\ref{fig:appendix-fig3-sd3-multi}, and Figure~\ref{fig:appendix-fig3-flux-multi}, the layer-wise cosine similarity patterns remain consistent across different model architectures, demonstrating the generalizability of our QR-LoRA framework. Specifically:

\begin{itemize}
    \item \textbf{$Q$ Matrix Properties:} Across all models, $Q$ matrices maintain remarkably high similarities (0.90-0.99), indicating their role as stable orthogonal bases for feature representation.
    \item \textbf{$R$ Matrix Characteristics:} The directly fine-tuned $R$ matrices show moderate but significant similarities (0.79-0.89), suggesting their inherited structural information from the original weights.
    \item \textbf{$\Delta R$ Matrix Behavior:} In contrast, $\Delta R$ matrices consistently exhibit substantially lower similarities (-0.17-0.25), validating their effectiveness in capturing task-specific features independently.
\end{itemize}

\begin{figure}[t]
    \centering
    \includegraphics[width=\linewidth]{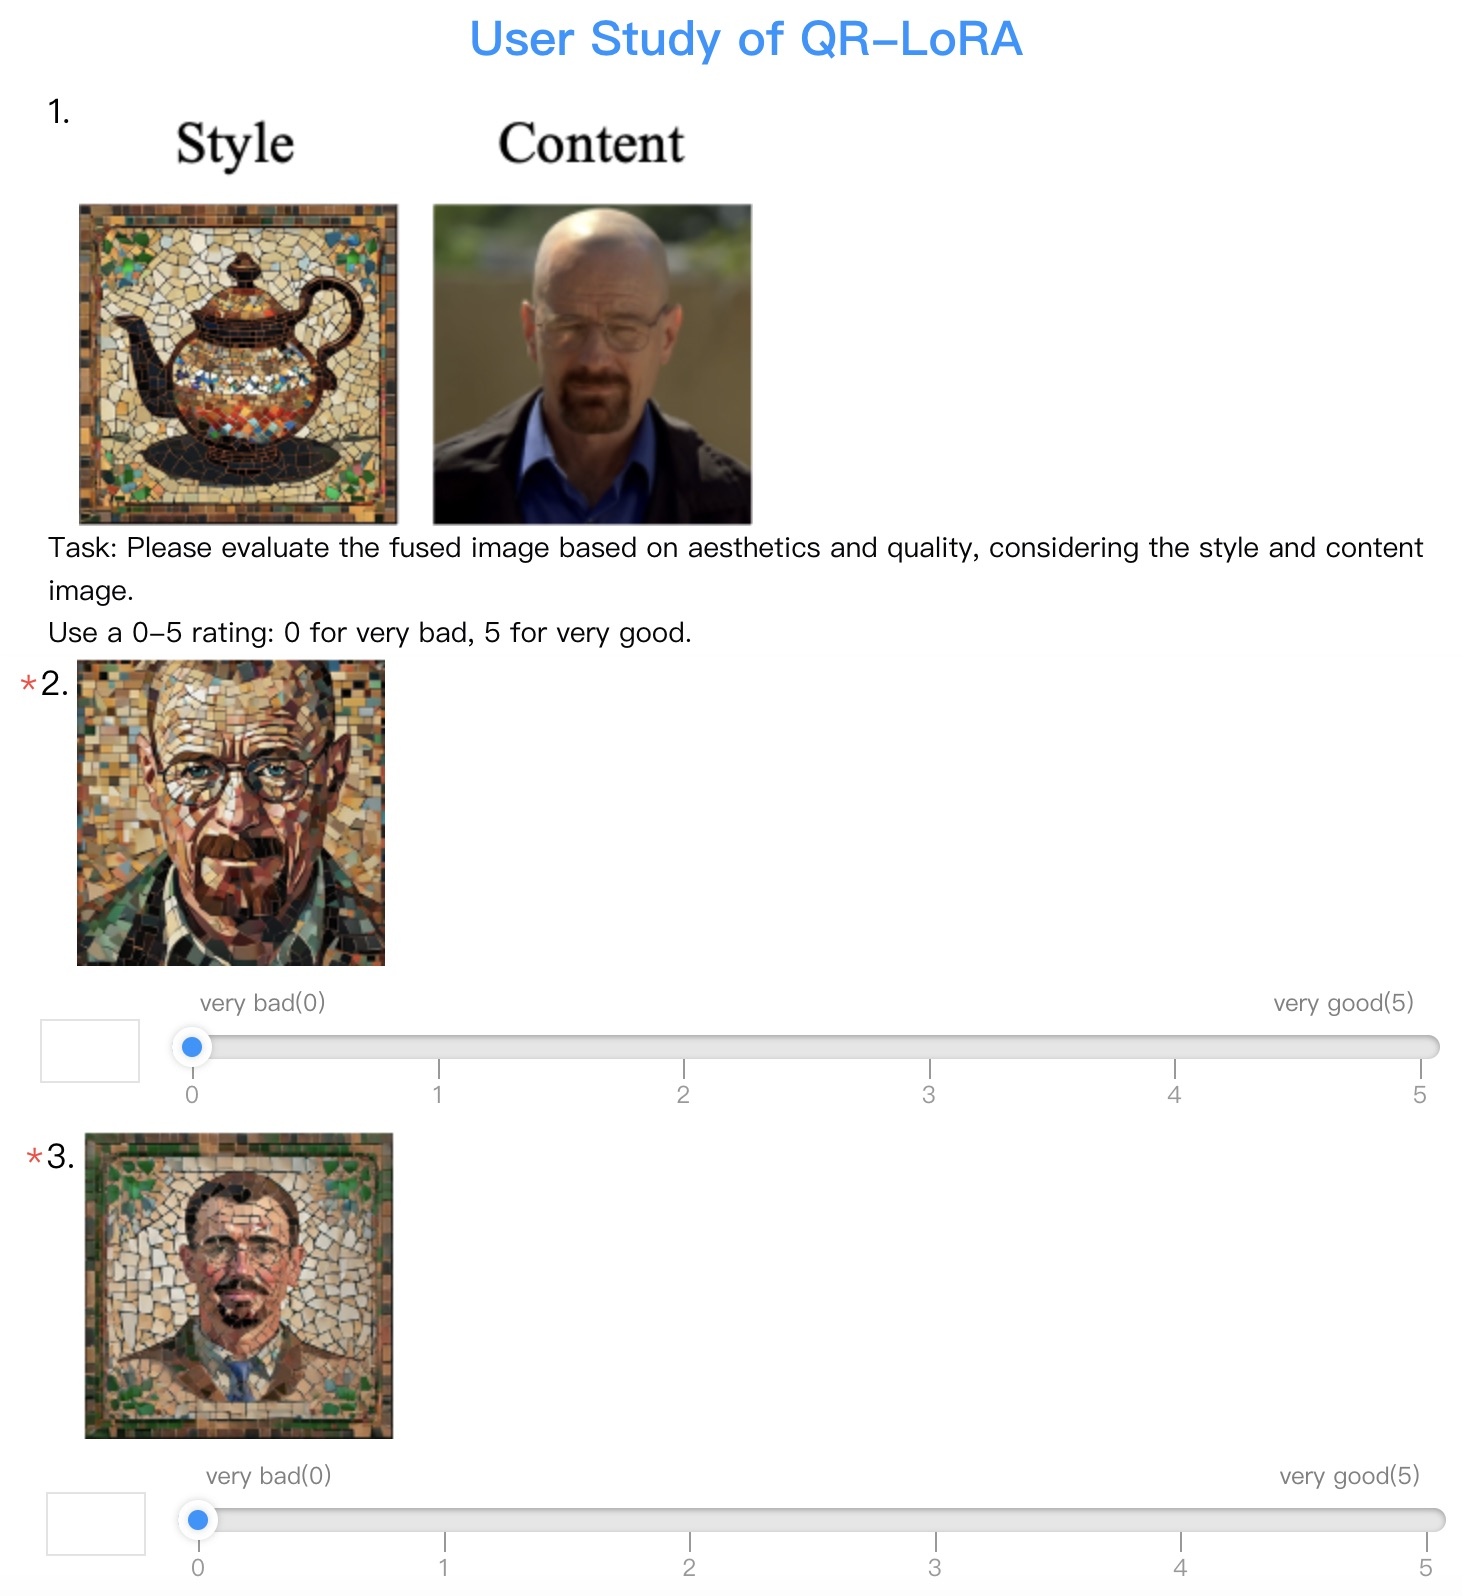}
    \caption{\textbf{User study interface.} Screenshot of our evaluation interface where participants rate generated images on a 0-5 scale based on content preservation and style transfer quality.}
    \label{fig:screenshot_of_user_study}
\end{figure}

\subsection{Statistical Analysis of Matrix Similarities}
The numerical results presented in Table~\ref{tab:matrix-similarity} provide a detailed quantitative perspective on the similarity patterns. The data reveals several key insights:

\begin{itemize}
    \item The maximum similarity values for $Q$ matrices consistently approach 1.0 (0.9998-0.9999), with minimum values remaining above 0.90, demonstrating the stability of the orthogonal basis.
    \item $R$ matrices show maximum similarities above 0.99 but with lower minimum values (0.79-0.89), reflecting their role in capturing task-relevant transformations while maintaining some degree of shared structure.
    \item $\Delta R$ matrices exhibit significantly lower similarity values, with maximums below 0.26 and minimums reaching -0.17, quantitatively confirming their capacity for independent feature representation.
    \item In comparison, traditional LoRA's $A$ matrices show consistently high similarities (0.77-1.0), while $B$ matrices display moderate to low similarities (0.15-0.38), highlighting the advantages of our orthogonal decomposition approach.
\end{itemize}

This comprehensive analysis validates the theoretical foundations of our QR-LoRA framework and demonstrates its effectiveness in achieving feature disentanglement across different model architectures. The consistent patterns observed in both layer-wise visualizations and statistical distributions support our design choice of focusing on $\Delta R$ updates for efficient and clean feature separation.

\begin{figure}[t]
    \centering
    \includegraphics[width=\linewidth]{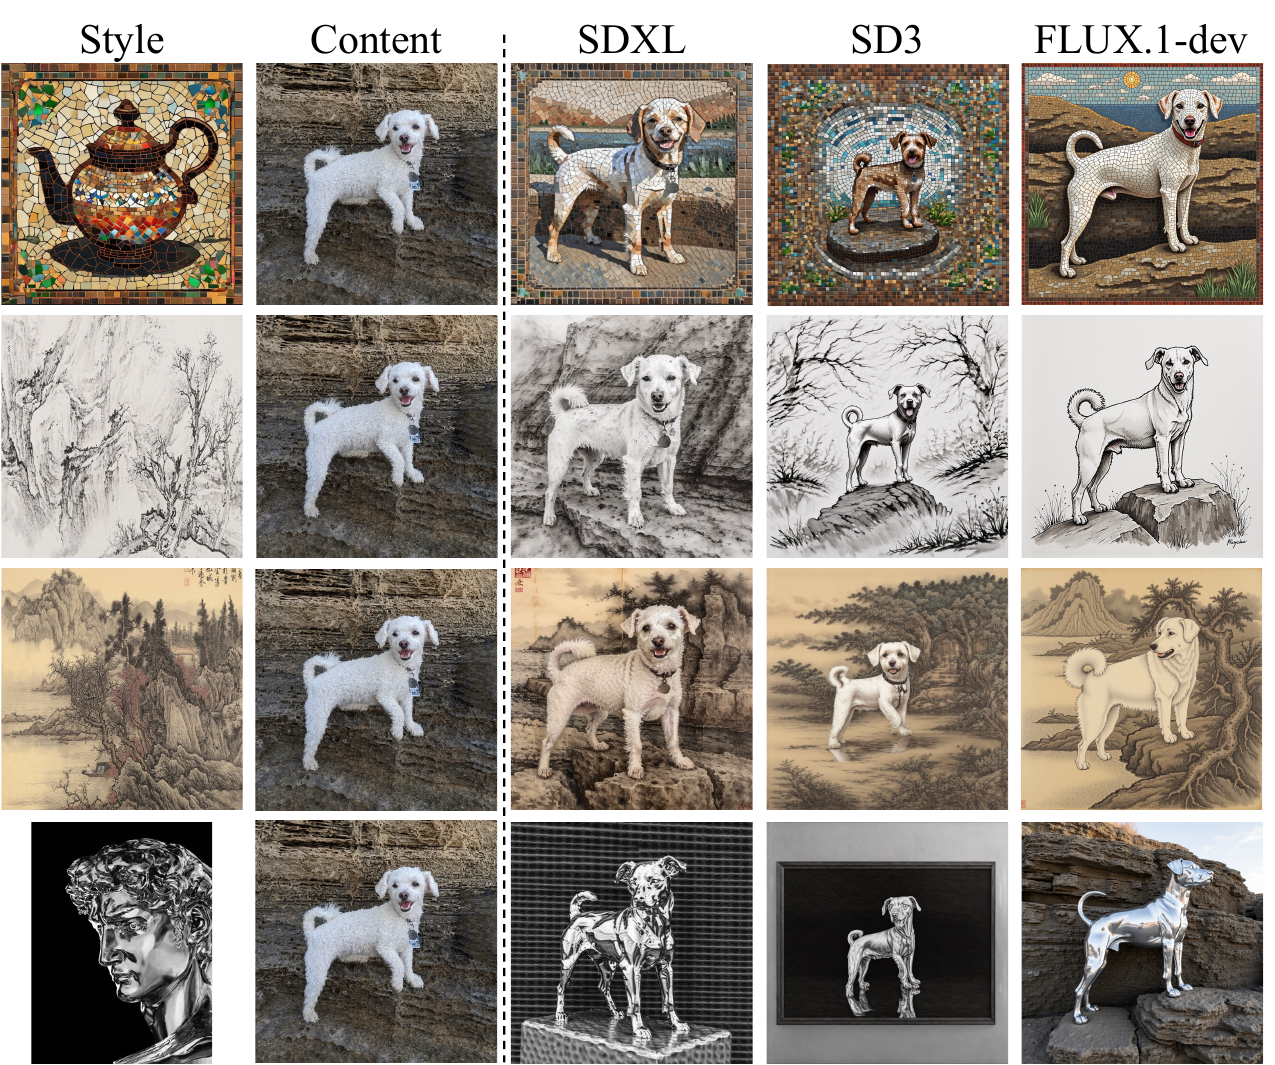}
        \caption{\textbf{Additional visualization results on different backbone models.} Extended demonstration of QR-LoRA's generation results across SDXL, SD3, and FLUX.1-dev models, further validating the consistent high-quality performance and model-agnostic nature of our approach. These supplementary examples provide a more comprehensive view of our method's capabilities across diverse model architectures, complementing the results presented in Figure~\ref{fig:vis_diff_backbones}.}
    \label{fig:appendix_vis_on_diff_backbone}
\end{figure}

\begin{figure*}[th]
    \centering
    \includegraphics[width=\linewidth]{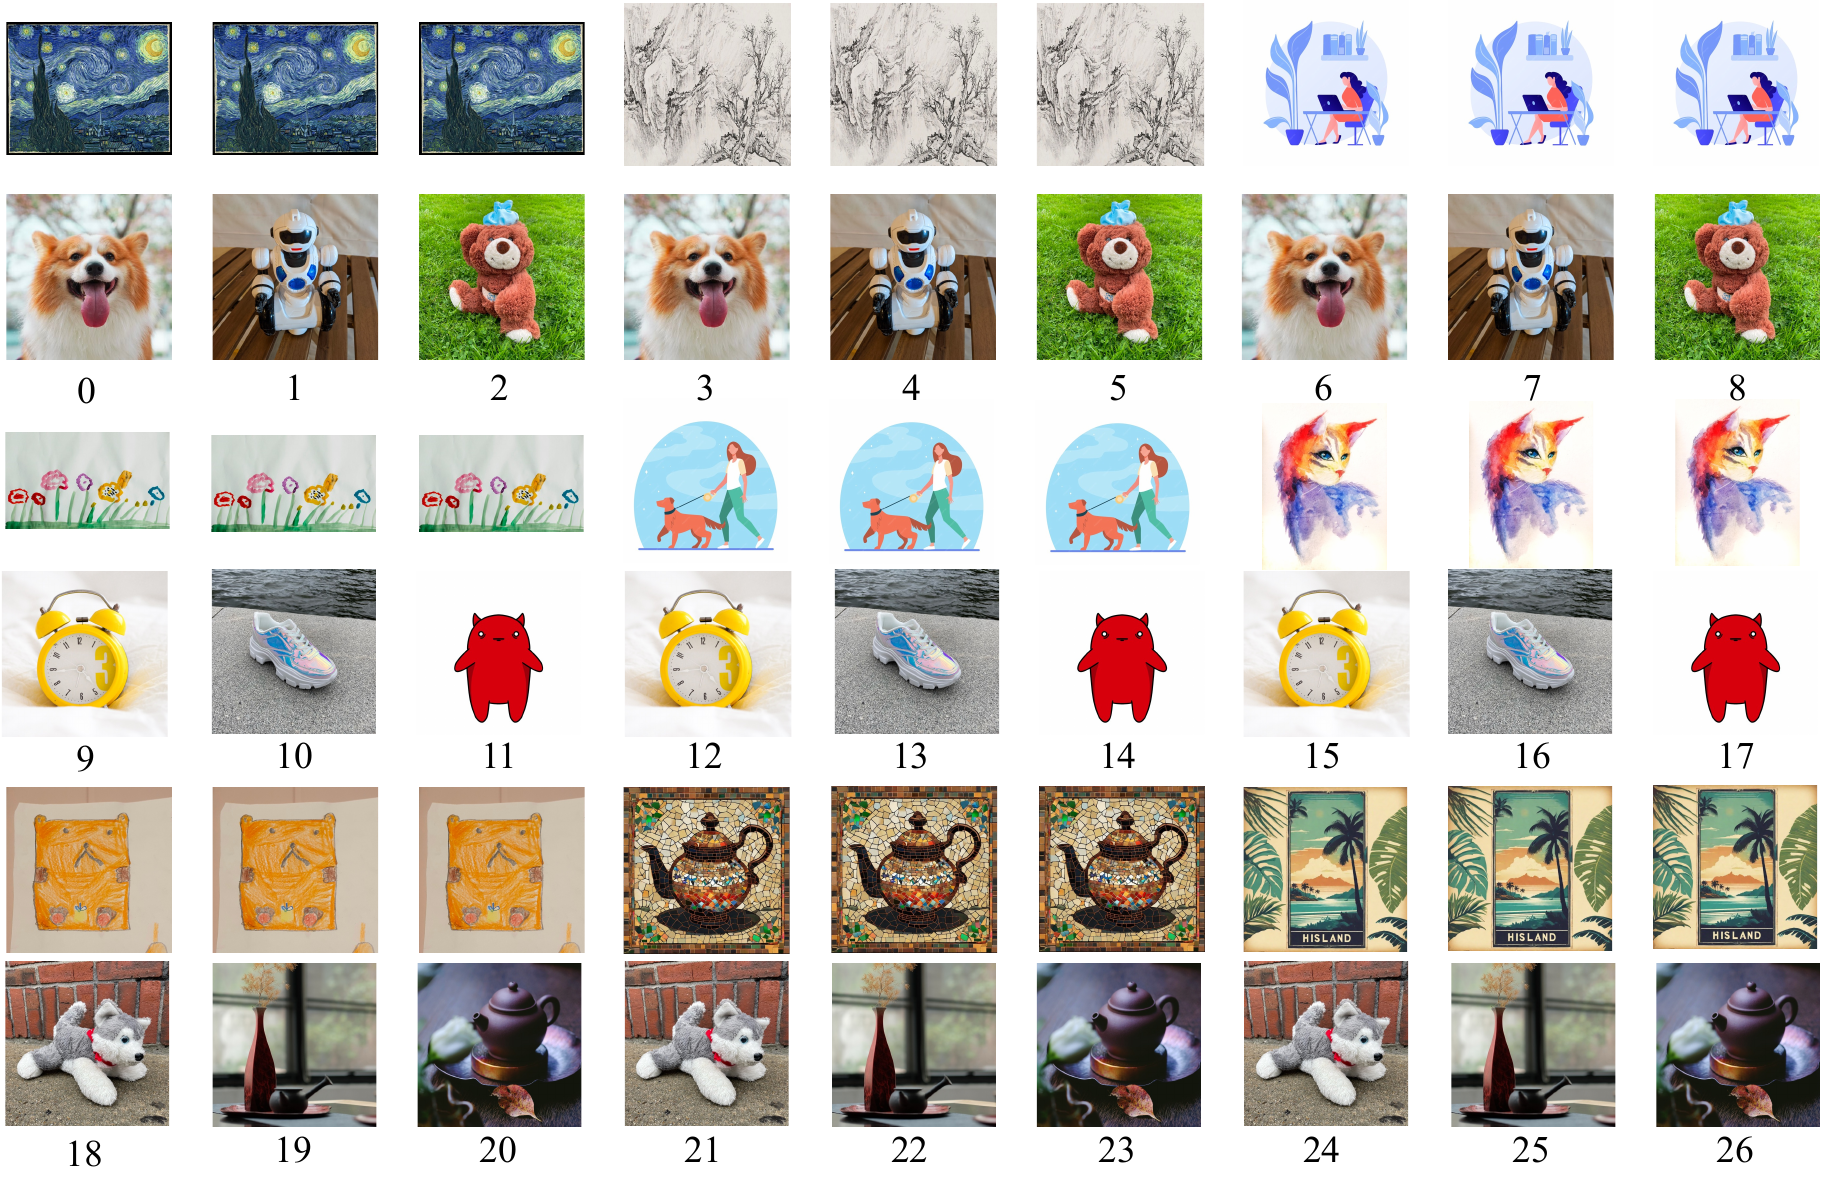}
    \caption{\textbf{Detailed experimental setup for matrix similarity comparison in Figure~\ref{fig:matrix-comparsion}.} We conduct experiments on 27 randomly selected image pairs to analyze the properties of different matrices in our QR-LoRA framework. For each image in the pairs, we train two types of LoRA adaptations: one using QR decomposition where both $Q$ and $R$ matrices are directly fine-tuned and another using the $\Delta R$ formulation. We then compute the cosine similarities between $Q$ matrices, $R$ matrices, and $\Delta R$ matrices across all injection layers in the SDXL model. 
    }
    % \vspace{-0.3cm}
    \label{fig:appendix-fig2}
\end{figure*}

\begin{table*}[]
\centering
\caption{\textbf{Numerical results of matrix similarity comparison in Figure~\ref{fig:matrix-comparsion}.} This table presents the detailed cosine similarity values for $Q$ matrices, $R$ matrices, $\Delta R$ matrices, $A$ matrices, and $B$ matrices from 27 pairs of image training data. For each image pair (\ie, sample index), we compute the cosine similarities across all injection layers in the SDXL model and record both the maximum ($Q_{max}$, $R_{max}$, $\Delta R_{max}$, $A_{max}$, $B_{max}$) and minimum ($Q_{min}$, $R_{min}$, $\Delta R_{min}$, $A_{min}$, $B_{min}$) similarity values. 
}
\label{tab:matrix-similarity}
\begin{tabular}{cllllllllll}
\toprule
\multicolumn{1}{c}{\textbf{Sample Index}} & \multicolumn{1}{c}{\textbf{$Q_{max}$}} & \multicolumn{1}{c}{\textbf{$Q_{min}$}} & \multicolumn{1}{c}{\textbf{$R_{max}$}} & \multicolumn{1}{c}{\textbf{$R_{min}$}} & \multicolumn{1}{c}{\textbf{$\Delta R_{max}$}} & \multicolumn{1}{c}{\textbf{$\Delta R_{min}$}} & \multicolumn{1}{c}{\textbf{$A_{max}$}} & \multicolumn{1}{c}{\textbf{$A_{min}$}} & \multicolumn{1}{c}{\textbf{$B_{max}$}} & \multicolumn{1}{c}{\textbf{$B_{min}$}} \\
\midrule
0 & 0.9999 & 0.9787 & 0.9997 & 0.8409 & 0.1657 & -0.1139 & 1.0000 & 0.8046 & 0.3615 & -0.0355 \\
1 & 0.9999 & 0.9786 & 0.9997 & 0.8253 & 0.1632 & -0.1223 & 1.0000 & 0.7970 & 0.3249 & -0.0625 \\
2 & 0.9999 & 0.9682 & 0.9997 & 0.8391 & 0.1135 & -0.1038 & 1.0000 & 0.8161 & 0.3198 & -0.0826 \\
3 & 0.9998 & 0.9311 & 0.9996 & 0.8104 & 0.1959 & -0.1335 & 1.0000 & 0.8075 & 0.2322 & -0.0565 \\
4 & 0.9998 & 0.9313 & 0.9996 & 0.7993 & 0.1241 & -0.0818 & 1.0000 & 0.8020 & 0.2295 & -0.0626 \\
5 & 0.9998 & 0.9055 & 0.9997 & 0.8143 & 0.1529 & -0.0872 & 1.0000 & 0.8144 & 0.2226 & -0.0558 \\
6 & 0.9998 & 0.9679 & 0.9997 & 0.8235 & 0.1566 & -0.0581 & 1.0000 & 0.7917 & 0.2113 & -0.0807 \\
7 & 0.9999 & 0.9680 & 0.9997 & 0.8129 & 0.1421 & -0.0699 & 1.0000 & 0.8126 & 0.2145 & -0.0783 \\
8 & 0.9999 & 0.9761 & 0.9997 & 0.8187 & 0.1257 & -0.0913 & 1.0000 & 0.8053 & 0.1898 & -0.2033 \\
9 & 0.9999 & 0.9709 & 0.9998 & 0.8441 & 0.1749 & -0.1036 & 1.0000 & 0.8272 & 0.3044 & -0.1188 \\
10 & 0.9999 & 0.9741 & 0.9998 & 0.8245 & 0.1500 & -0.0783 & 1.0000 & 0.8163 & 0.2070 & -0.0793 \\
11 & 0.9999 & 0.9792 & 0.9998 & 0.8833 & 0.1399 & -0.0611 & 1.0000 & 0.8379 & 0.1525 & -0.1278 \\
12 & 0.9999 & 0.9765 & 0.9997 & 0.8485 & 0.1816 & -0.1094 & 1.0000 & 0.8253 & 0.2499 & -0.0961 \\
13 & 0.9999 & 0.9793 & 0.9998 & 0.8216 & 0.2493 & -0.0463 & 1.0000 & 0.8164 & 0.1490 & -0.1374 \\
14 & 0.9999 & 0.9854 & 0.9999 & 0.8894 & 0.2067 & -0.0933 & 1.0000 & 0.8332 & 0.1817 & -0.1316 \\
15 & 0.9998 & 0.9724 & 0.9996 & 0.8410 & 0.1756 & -0.1686 & 1.0000 & 0.8416 & 0.3820 & -0.0801 \\
16 & 0.9998 & 0.9752 & 0.9996 & 0.8186 & 0.1851 & -0.1050 & 1.0000 & 0.8361 & 0.2329 & -0.0636 \\
17 & 0.9998 & 0.9807 & 0.9997 & 0.8818 & 0.1262 & -0.0695 & 1.0000 & 0.8413 & 0.2125 & -0.1462 \\
18 & 0.9999 & 0.9055 & 0.9996 & 0.8340 & 0.2539 & -0.0760 & 1.0000 & 0.8346 & 0.3847 & -0.2045 \\
19 & 0.9999 & 0.9054 & 0.9997 & 0.8408 & 0.1209 & -0.0420 & 1.0000 & 0.8398 & 0.2905 & -0.0762 \\
20 & 0.9999 & 0.9053 & 0.9996 & 0.8339 & 0.1705 & -0.0540 & 1.0000 & 0.8298 & 0.2734 & -0.0548 \\
21 & 0.9998 & 0.9045 & 0.9995 & 0.8040 & 0.2042 & -0.0466 & 1.0000 & 0.7727 & 0.1746 & -0.0739 \\
22 & 0.9998 & 0.9044 & 0.9995 & 0.8095 & 0.1441 & -0.0716 & 1.0000 & 0.7714 & 0.1531 & -0.1031 \\
23 & 0.9998 & 0.9045 & 0.9995 & 0.7992 & 0.1473 & -0.0588 & 1.0000 & 0.7853 & 0.1558 & -0.0861 \\
24 & 0.9998 & 0.9055 & 0.9996 & 0.8272 & 0.1711 & -0.0512 & 1.0000 & 0.8034 & 0.1969 & -0.0806 \\
25 & 0.9998 & 0.9053 & 0.9996 & 0.8207 & 0.1686 & -0.0851 & 1.0000 & 0.8147 & 0.2685 & -0.0401 \\
26 & 0.9998 & 0.9053 & 0.9996 & 0.8134 & 0.1719 & -0.0850 & 1.0000 & 0.8108 & 0.2691 & -0.0488 \\
\bottomrule
\end{tabular}
\end{table*}

\begin{figure*}[th]
    \centering
    \includegraphics[width=\linewidth]{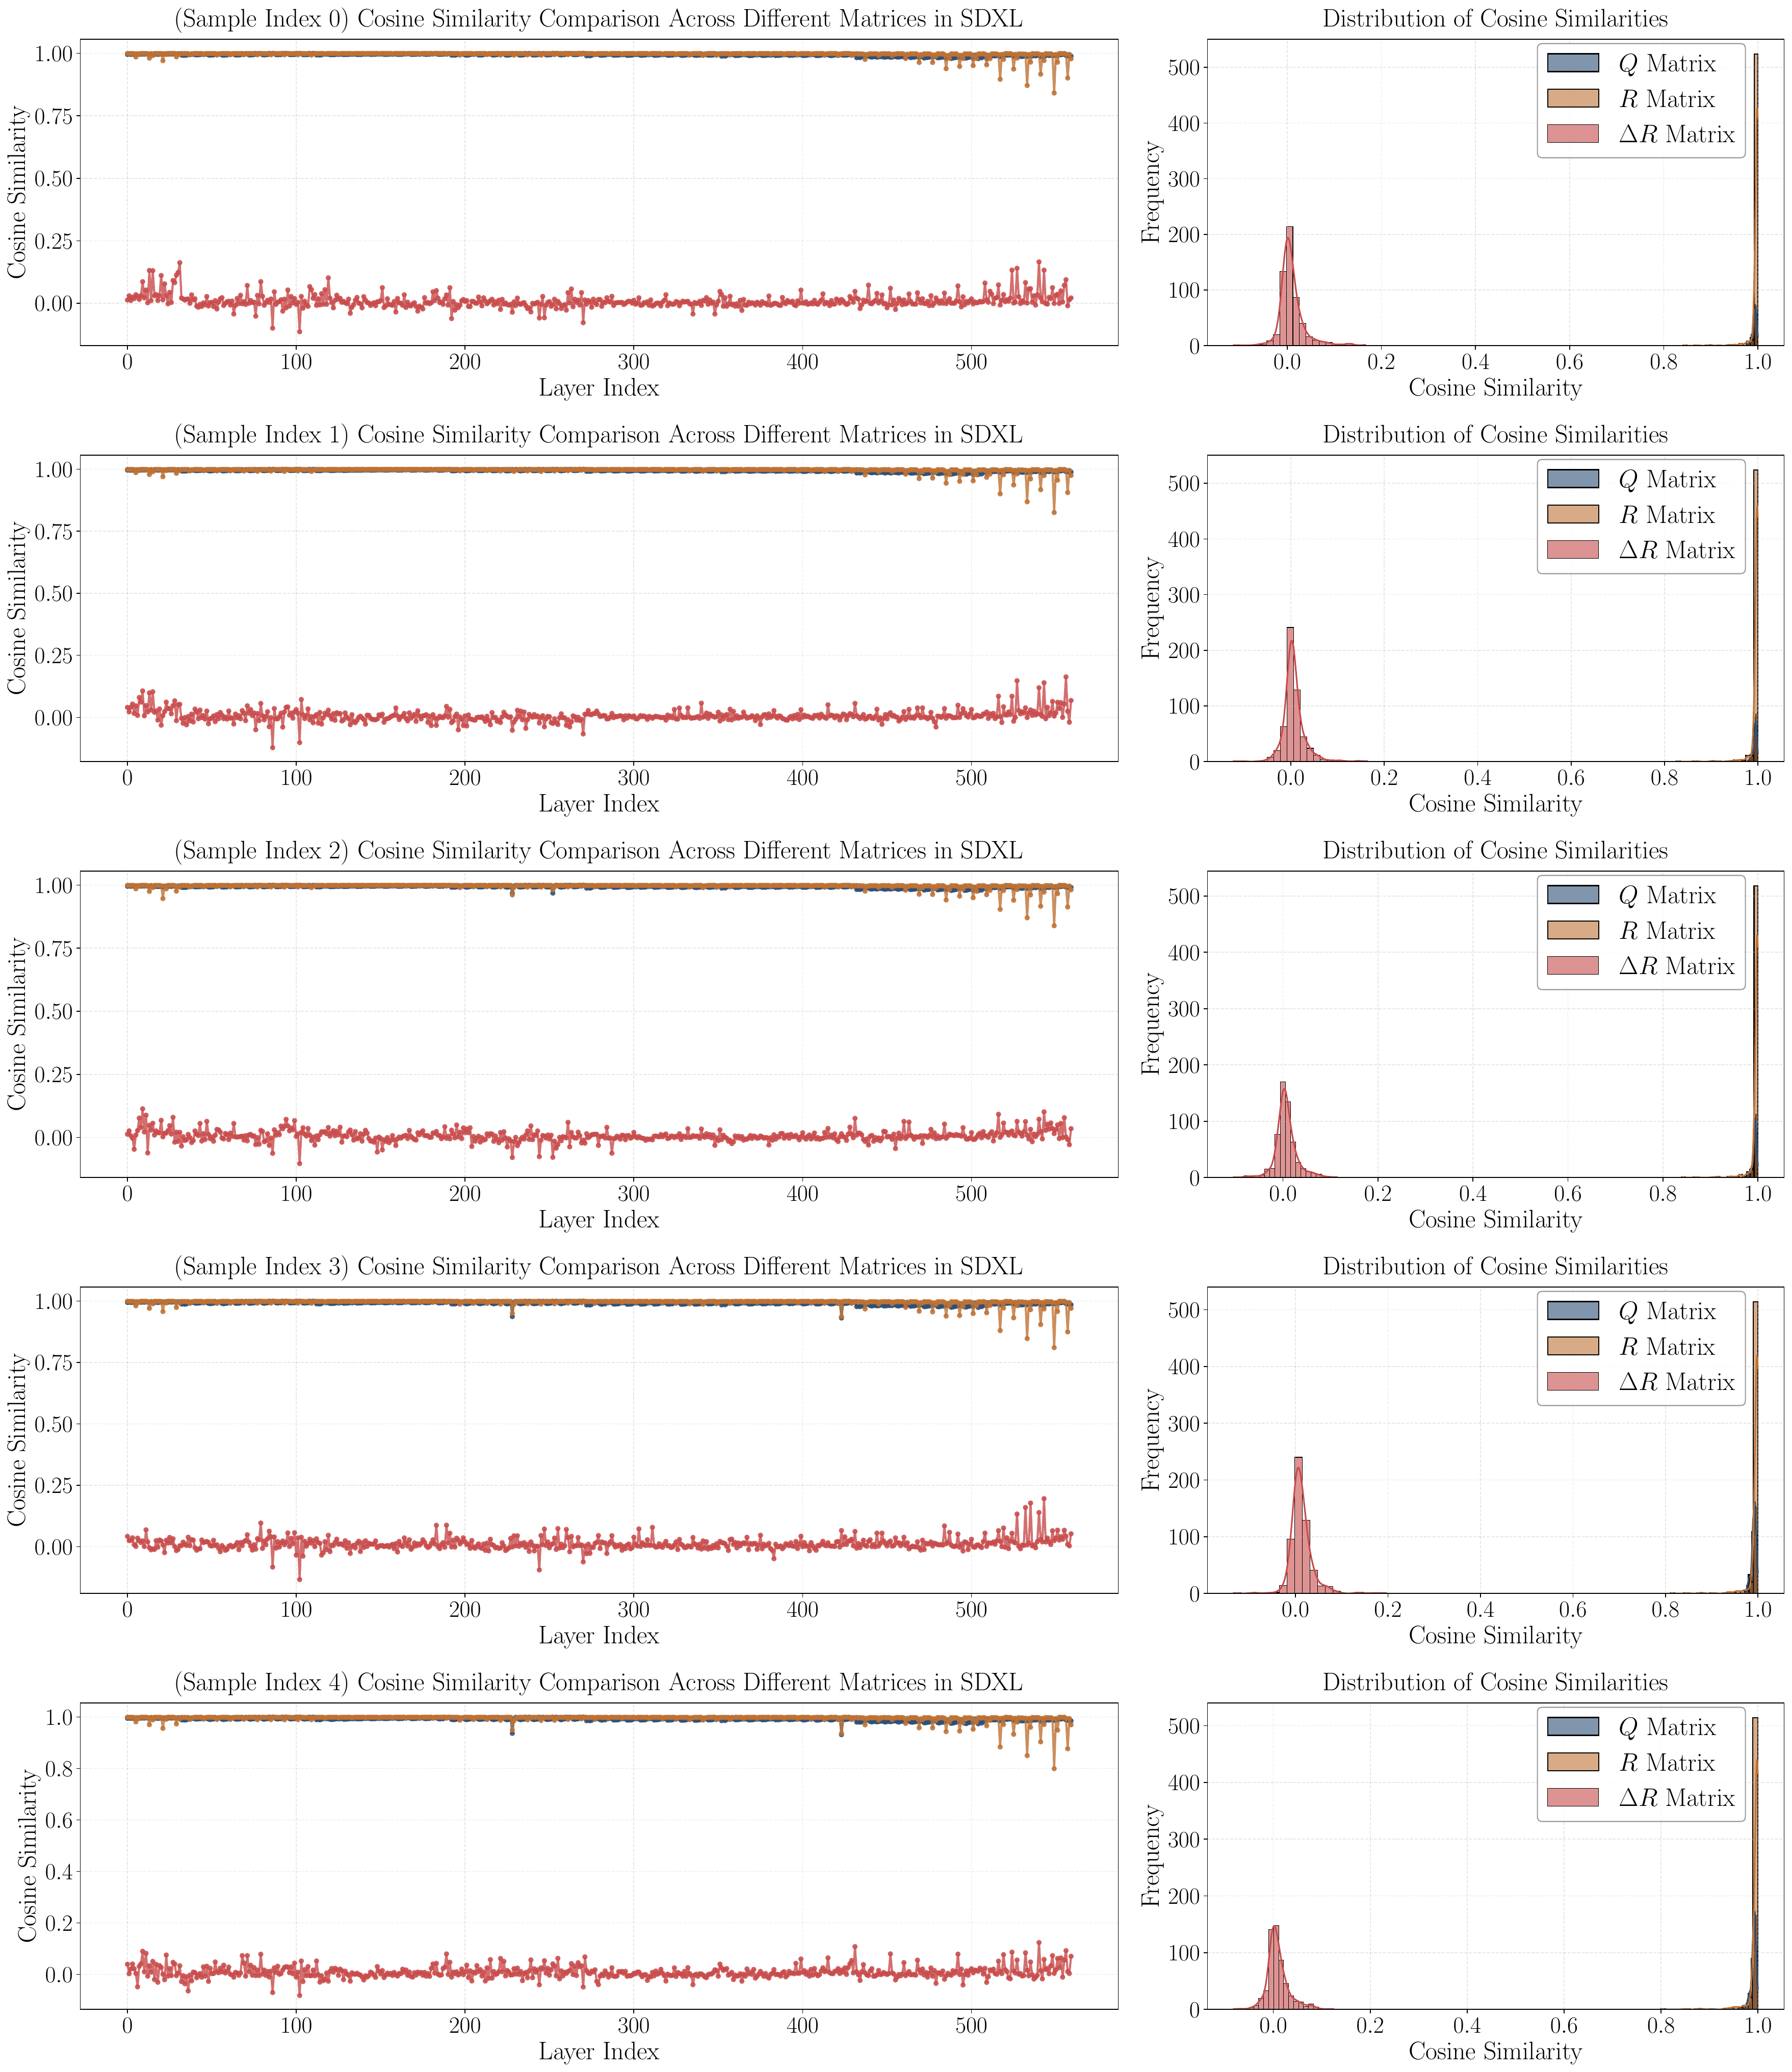}
    \caption{\textbf{Extended analysis of cosine similarities under SDXL model, complementing Figure~\ref{fig:matrix-detail-comparsion-in-sdxl}.} We replicate the similarity analysis experiment (sample index from 0 to 4) from Figure~\ref{fig:matrix-detail-comparsion-in-sdxl} using the SDXL backbone model to validate the generalization of our findings. The left panel shows the layer-wise cosine similarity trends across different training strategies, consistent with our main results. Additionally, we provide histogram distributions of similarity values in the right panel, offering a statistical perspective on the similarity patterns. This comprehensive visualization further supports our theoretical analysis by demonstrating that the observed matrix properties are consistent across different model architectures.
    }
    % \vspace{-0.3cm}
    \label{fig:appendix-fig3-sdxl-multi}
\end{figure*}

\begin{figure*}[th]
    \centering
    \includegraphics[width=\linewidth]{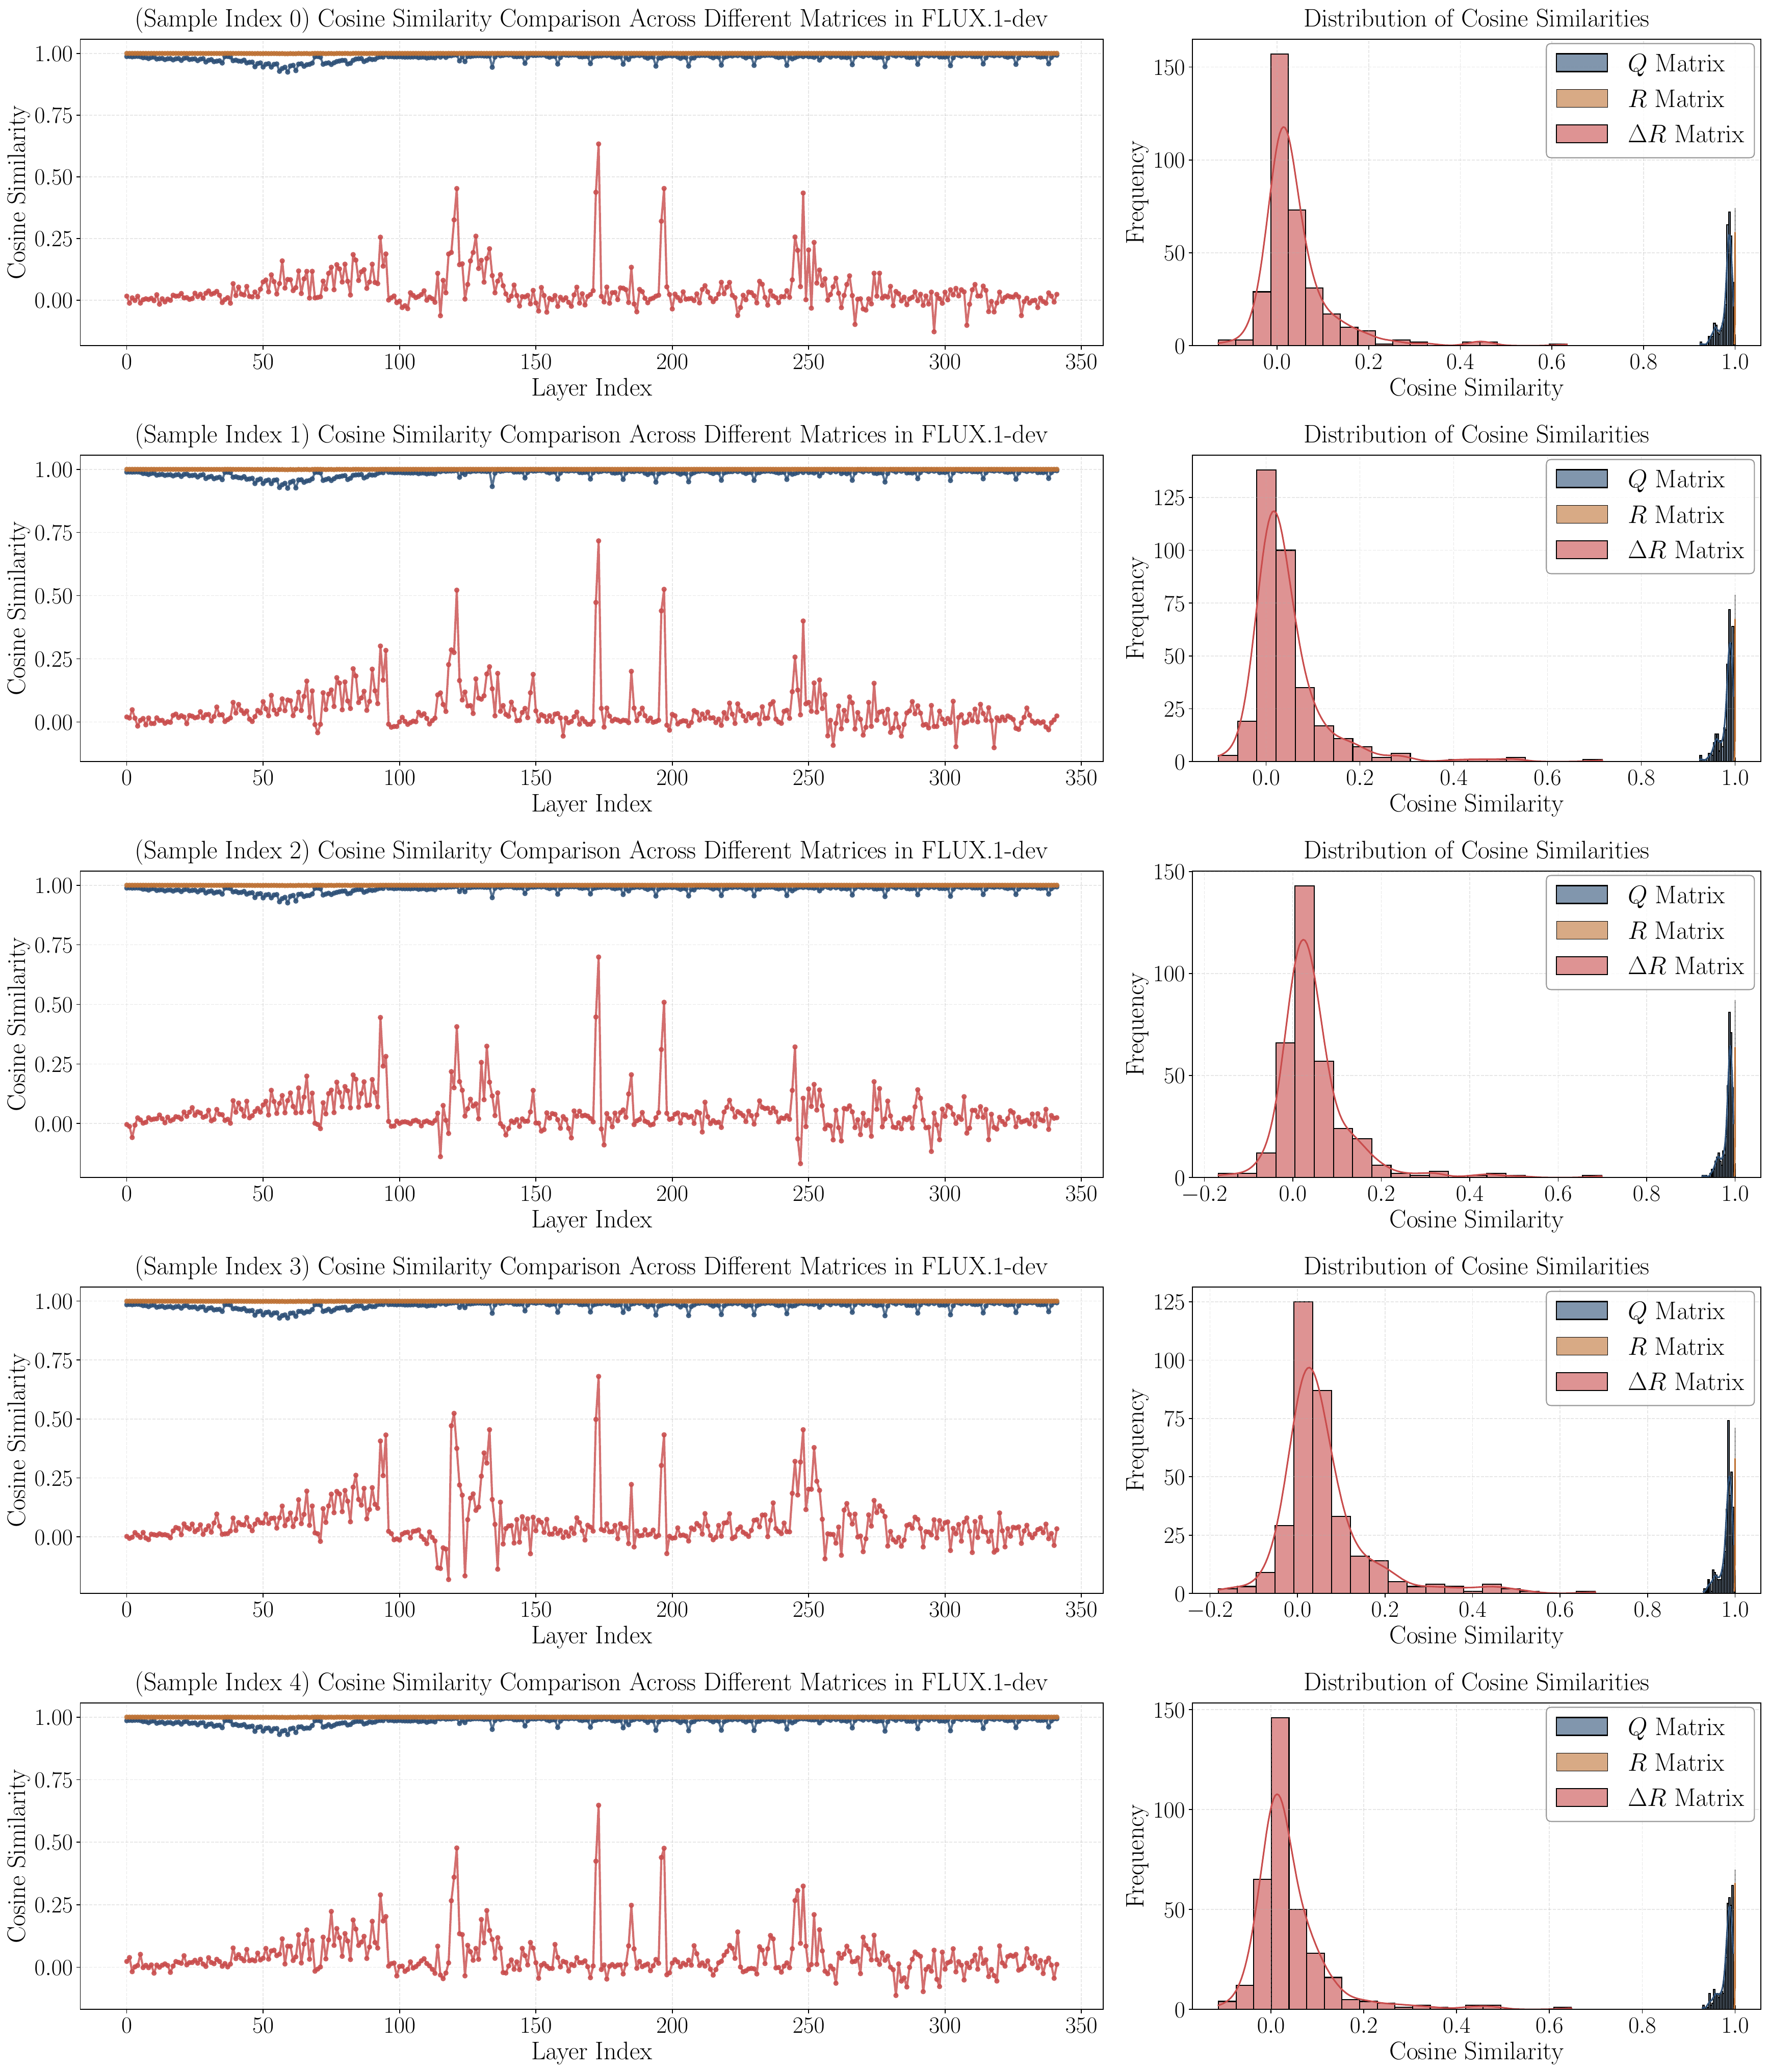}
    \caption{\textbf{Extended analysis of cosine similarities under FLUX.1-dev model, complementing Figure~\ref{fig:matrix-detail-comparsion-in-sdxl}.} We replicate the similarity analysis experiment (sample index from 0 to 4) from Figure~\ref{fig:matrix-detail-comparsion-in-sdxl} using the FLUX.1-dev backbone model to validate the generalization of our findings. The left panel shows the layer-wise cosine similarity trends across different training strategies, consistent with our main results. Additionally, we provide histogram distributions of similarity values in the right panel, offering a statistical perspective on the similarity patterns. This comprehensive visualization further supports our theoretical analysis by demonstrating that the observed matrix properties are consistent across different model architectures.
    }
    % \vspace{-0.3cm}
    \label{fig:appendix-fig3-flux-multi}
\end{figure*}

\begin{figure*}[th]
    \centering
    \includegraphics[width=\linewidth]{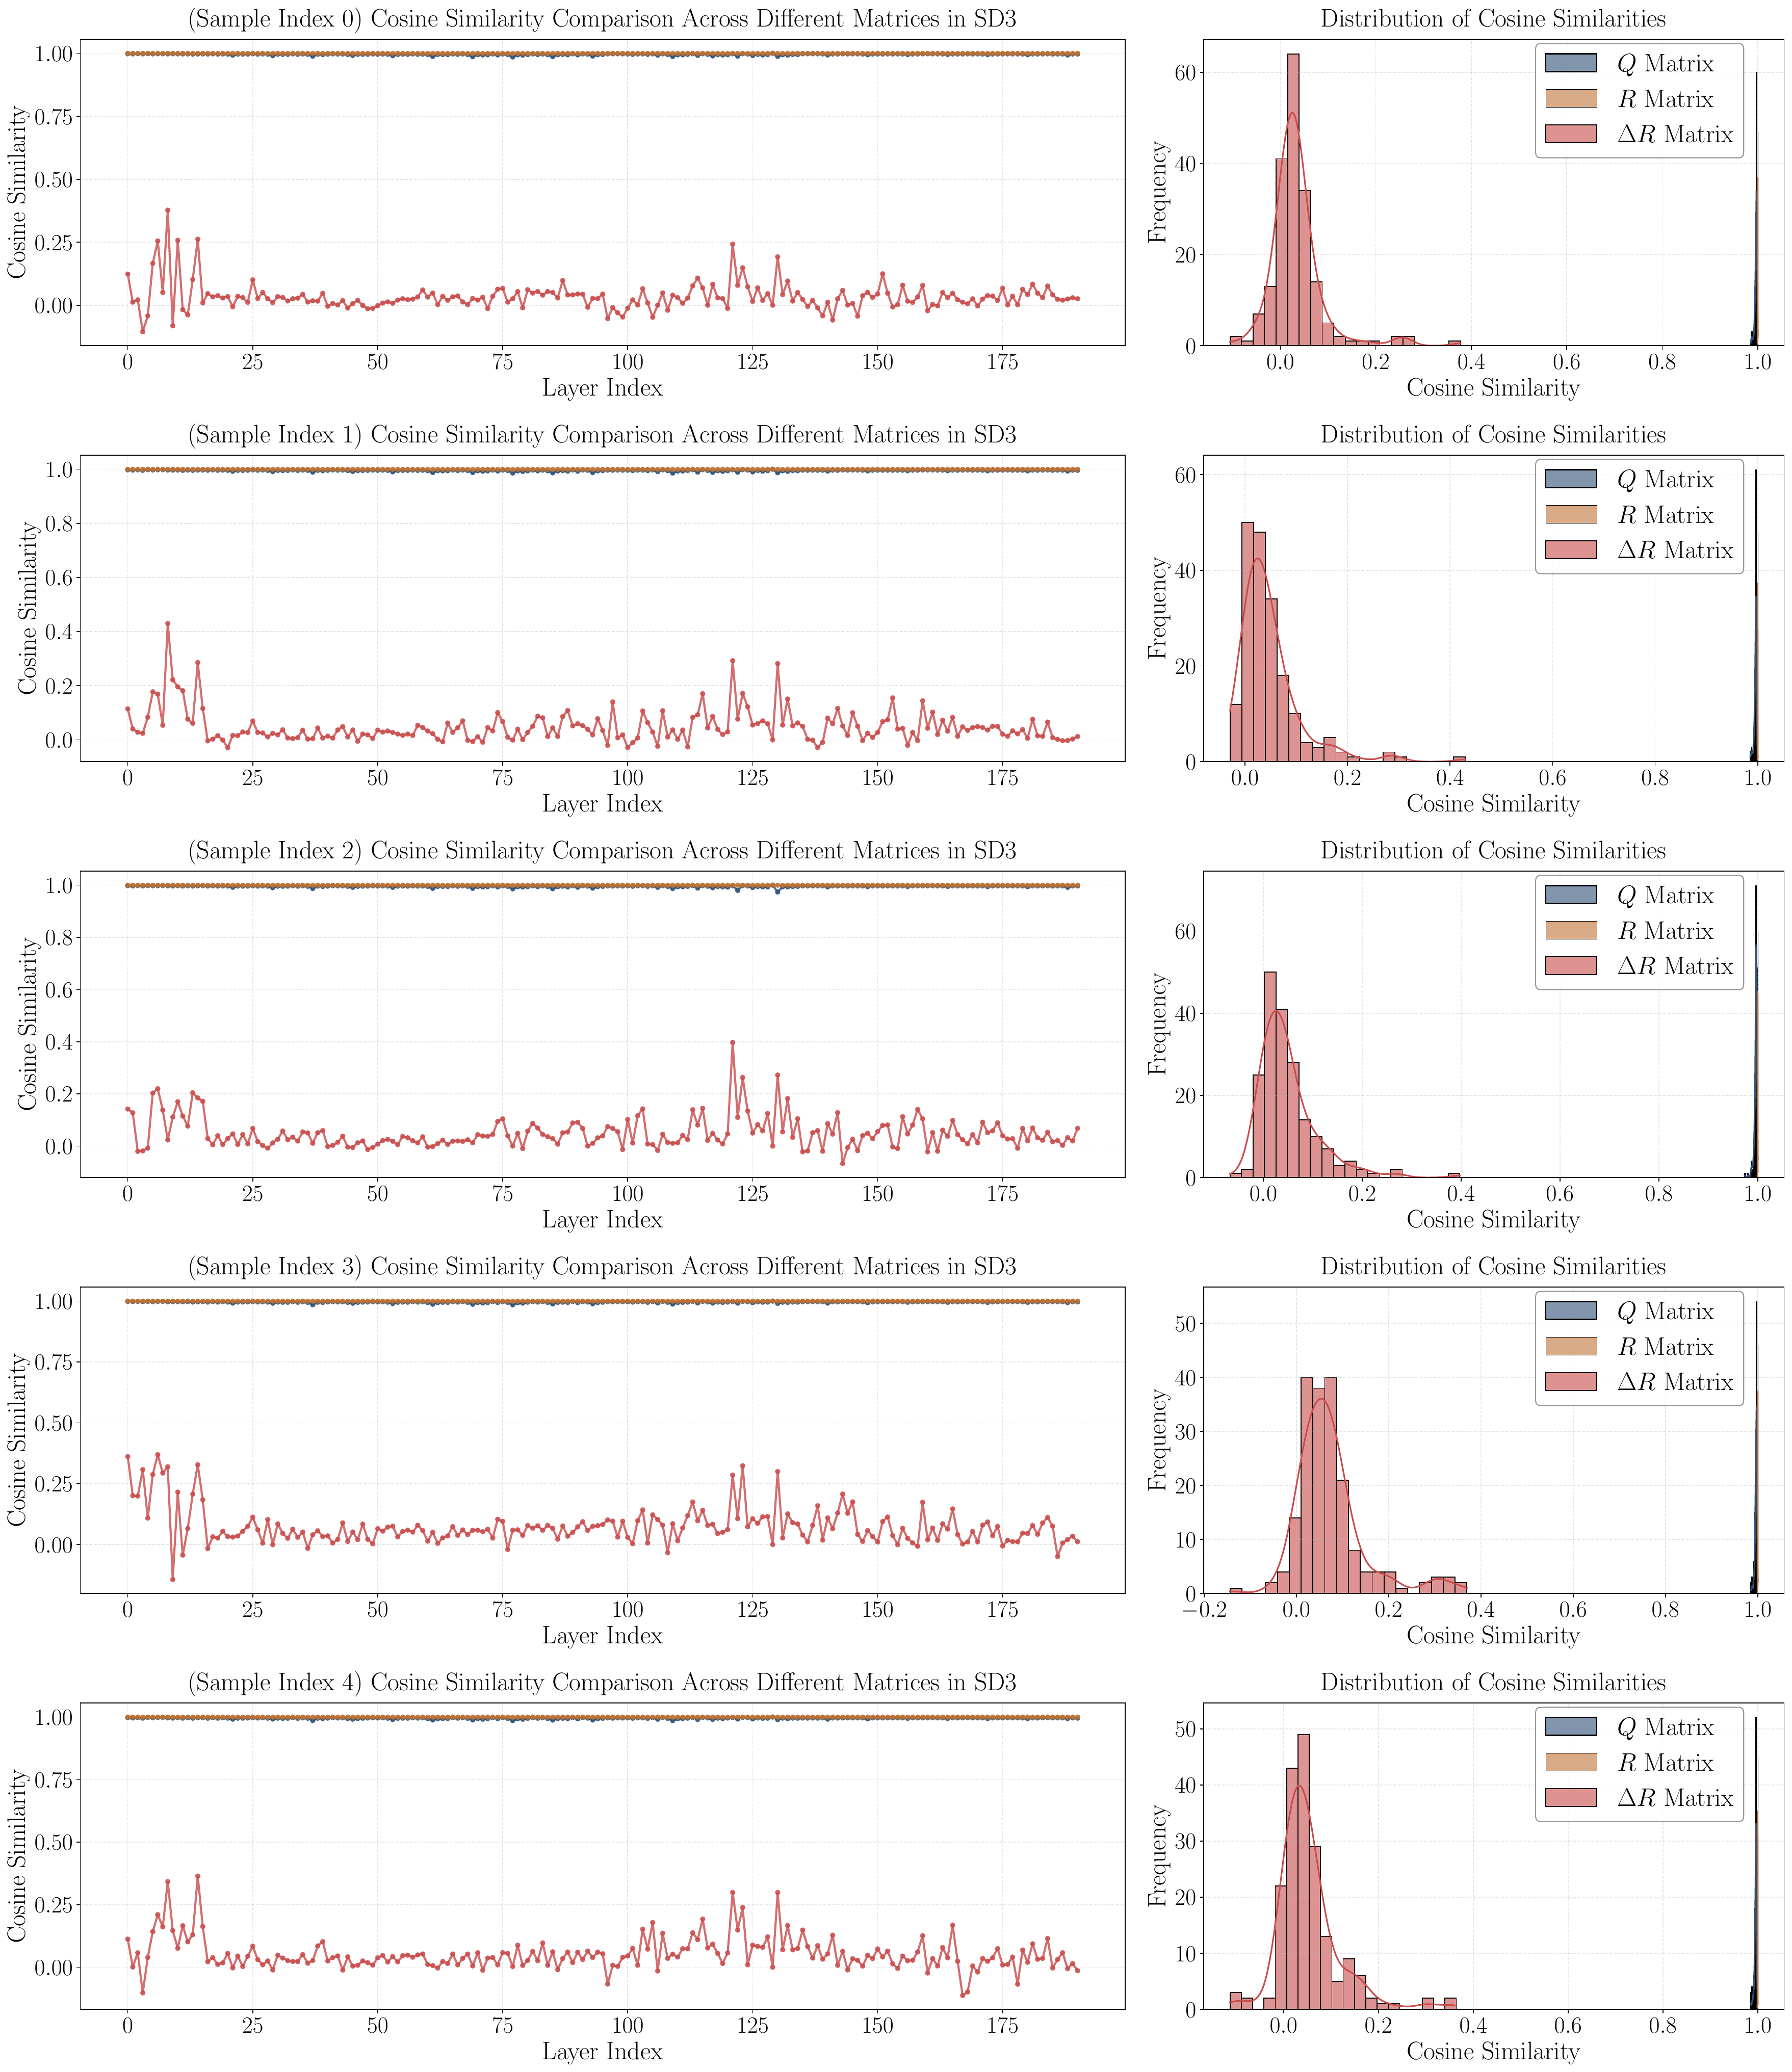}
    \caption{\textbf{Extended analysis of cosine similarities under SD3 model, complementing Figure~\ref{fig:matrix-detail-comparsion-in-sdxl}.} We replicate the similarity analysis experiment (sample index from 0 to 4) from Figure~\ref{fig:matrix-detail-comparsion-in-sdxl} using the SD3 backbone model to validate the generalization of our findings. The left panel shows the layer-wise cosine similarity trends across different training strategies, consistent with our main results. Additionally, we provide histogram distributions of similarity values in the right panel, offering a statistical perspective on the similarity patterns. This comprehensive visualization further supports our theoretical analysis by demonstrating that the observed matrix properties are consistent across different model architectures.
    }
    % \vspace{-0.3cm}
    \label{fig:appendix-fig3-sd3-multi}
\end{figure*}

\section{Additional Experimental Results and Discussion}

\subsection{Ablation Studies}
\textbf{Scaling coefficient.}
To comprehensively evaluate the robustness and flexibility of our QR-LoRA framework, we conduct extensive ablation studies on scaling coefficients across three different backbone models: SDXL, SD3, and FLUX.1-dev. Our experiments systematically explore coefficient combinations (\ie, $\lambda_c,\lambda_s$) ranging from 0.5 to 1.0 with intervals of 0.1, resulting in 36 distinct combinations for each model. This granular analysis reveals several key insights about our method's behavior and capabilities.

As demonstrated in Figures~\ref{fig:appendix-ablation-coeff-sdxl}, \ref{fig:appendix-ablation-coeff-sd3}, and \ref{fig:appendix-ablation-coeff-flux}, our approach maintains consistent generation quality across different coefficient settings while enabling fine-grained control over the content-style fusion process. The smooth transitions observed between different coefficient combinations indicate that our QR decomposition effectively disentangles content and style features, allowing for intuitive and stable interpolation between these attributes. Notably, this behavior remains consistent across all three model architectures, validating the model-agnostic nature of our approach.

Furthermore, our experiments demonstrate that our method exhibits robust performance across a wide range of scaling coefficients after obtaining the disentangled deltaR matrices. This scaling exploration serves as a deeper investigation into our method's capabilities, rather than a limitation. It's worth noting that such scaling strategies are generally applicable to any LoRA-based methods, showcasing the versatility of our approach in achieving various levels of content preservation and style transfer effects.

\textbf{Rank.}
To comprehensively evaluate the robustness of our method, we conduct a sensitivity analysis across different rank settings. As shown in Figure~\ref{fig:rank_ablation}, our method demonstrates consistent performance and stable generation quality across various rank values, indicating its inherent robustness to this hyperparameter. We adopt rank=64 for all experiments in the main paper, as it strikes an optimal balance between computational efficiency and generation quality. This choice aligns well with common practices in the literature \cite{shah2025ziplora,frenkel2025blora} and proves to be a reliable setting for most applications.

\begin{figure*}[th]
    \centering
    \includegraphics[width=\linewidth]{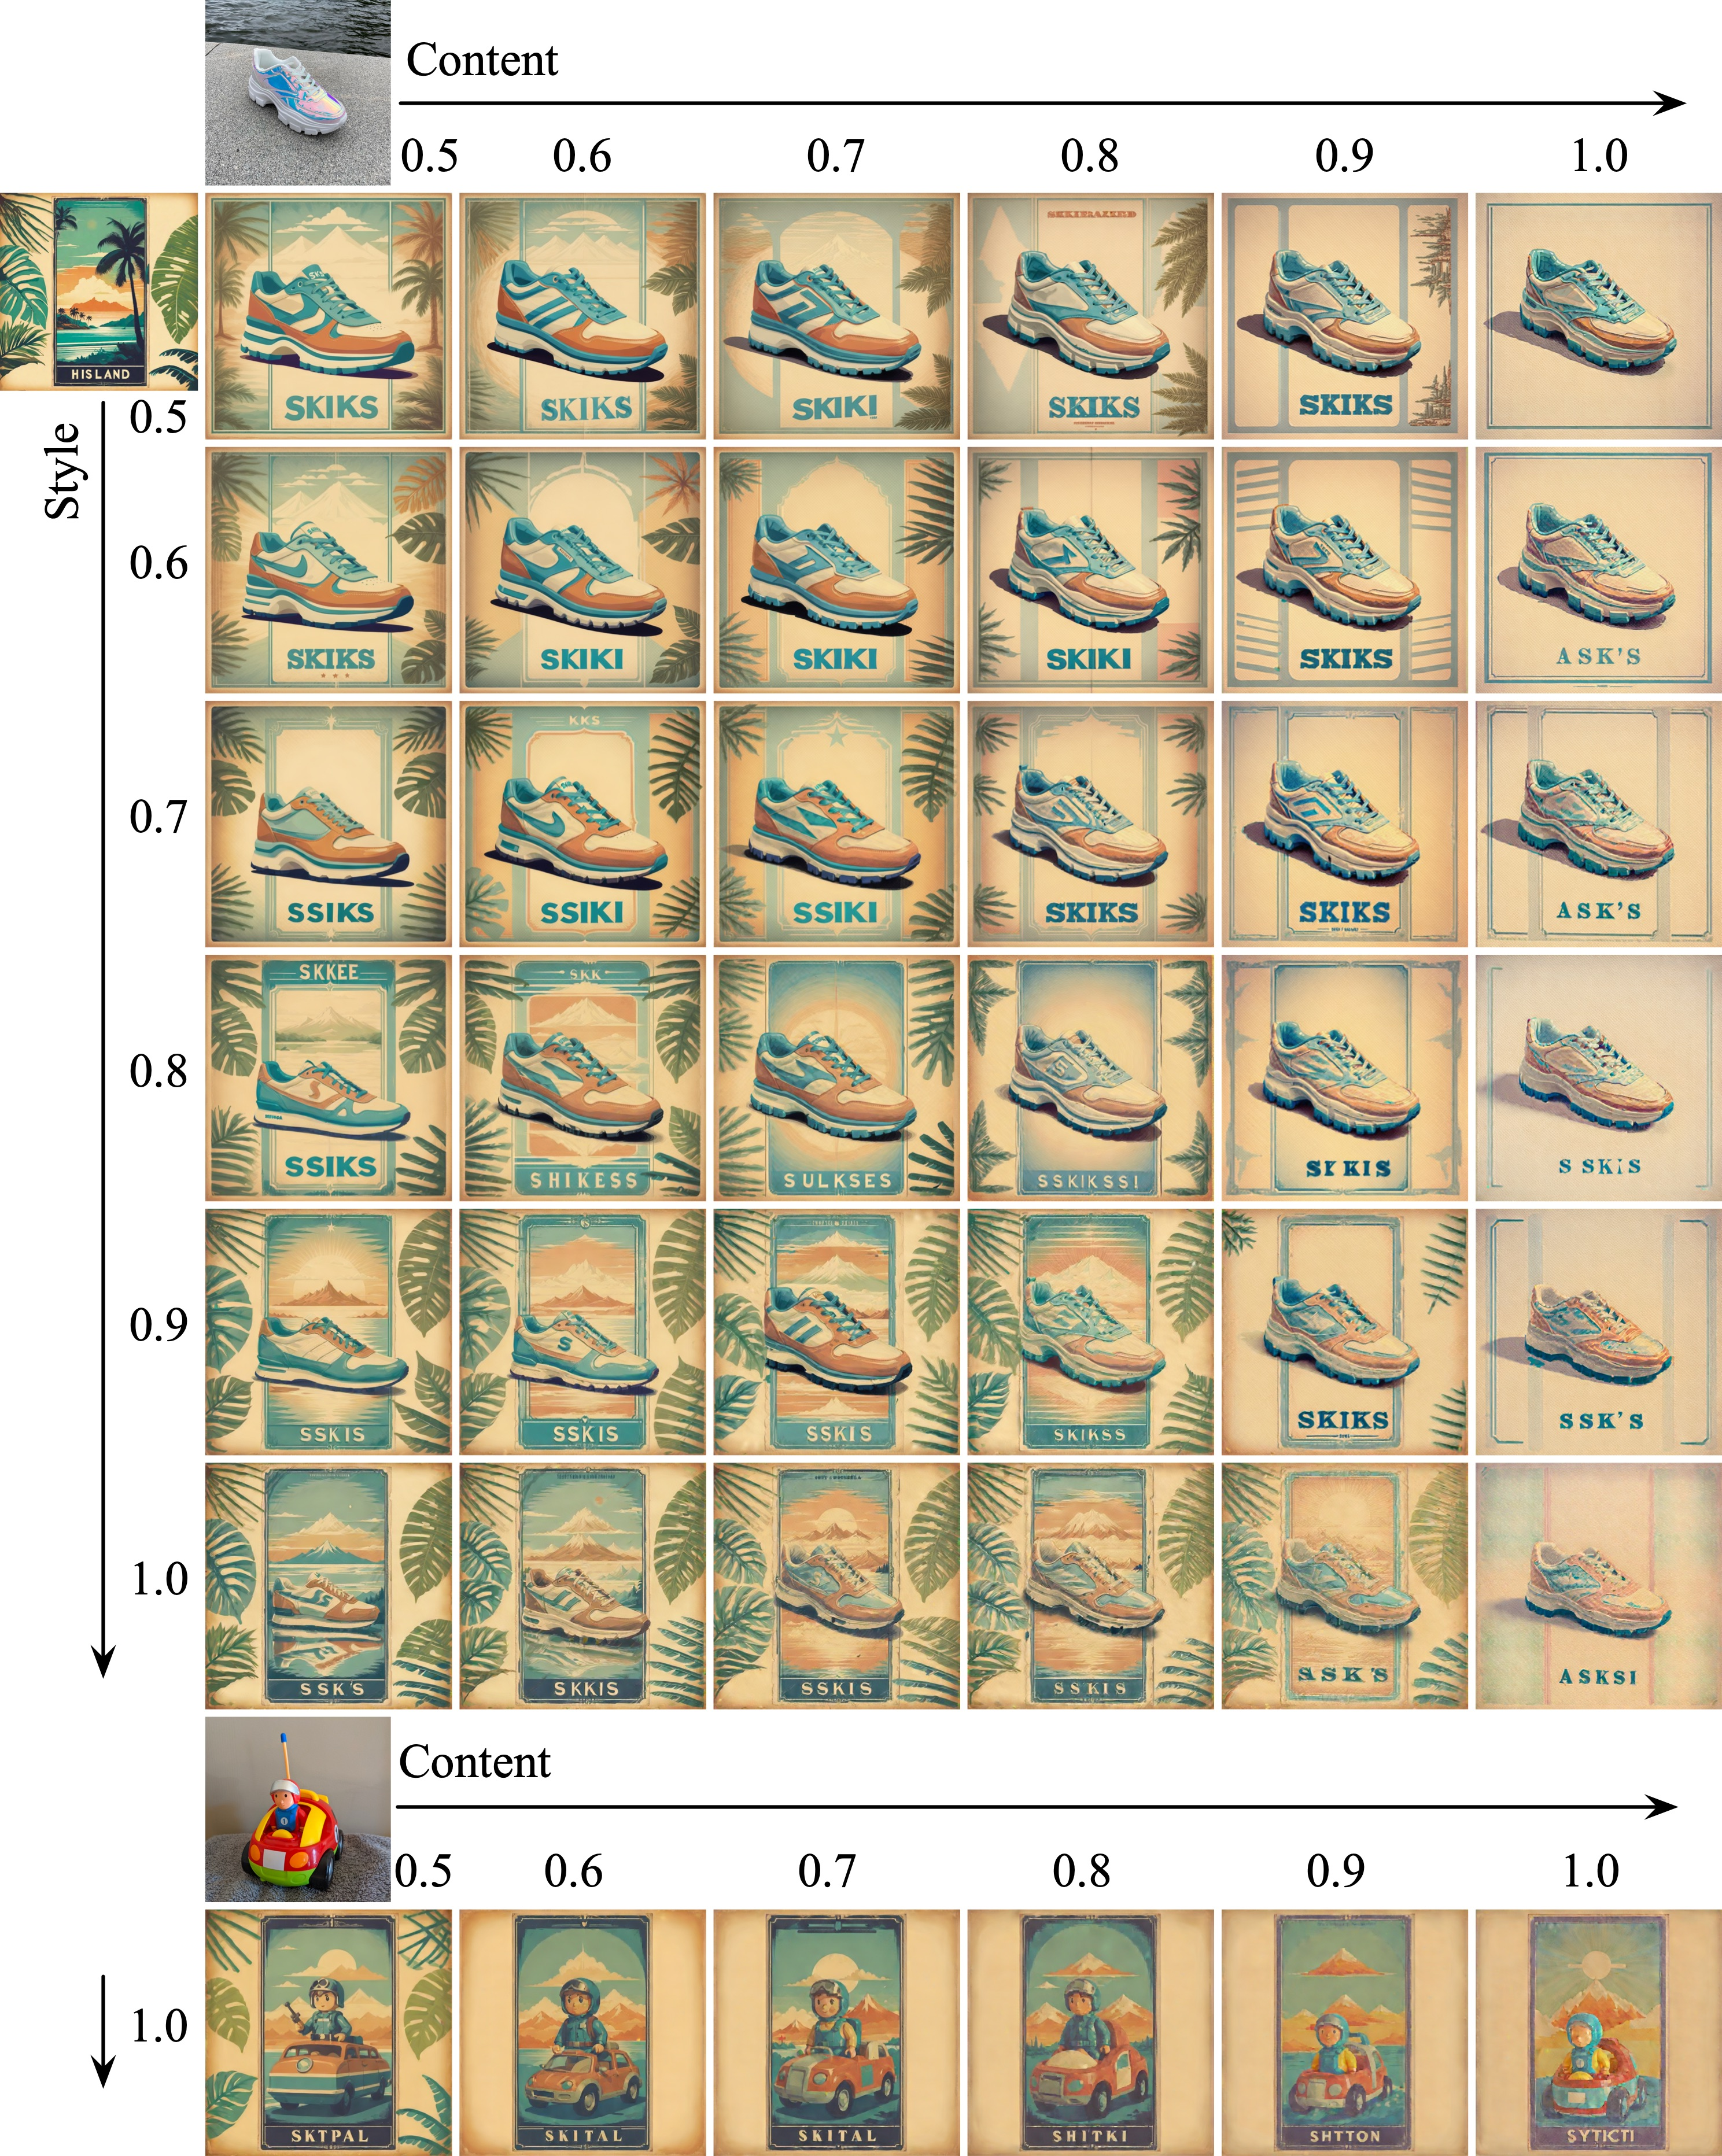}
    \caption{\textbf{Comprehensive ablation study on scaling coefficients for content-style fusion based on SDXL.} We demonstrate the generation results under various combinations of content and style scaling coefficients. The experiments validate the flexibility and robustness of our approach in achieving fine-grained control over content-style fusion through different coefficient combinations. Please zoom in to view details.}
    \label{fig:appendix-ablation-coeff-sdxl}
\end{figure*}

\begin{figure*}[th]
    \centering
    \includegraphics[width=\linewidth]{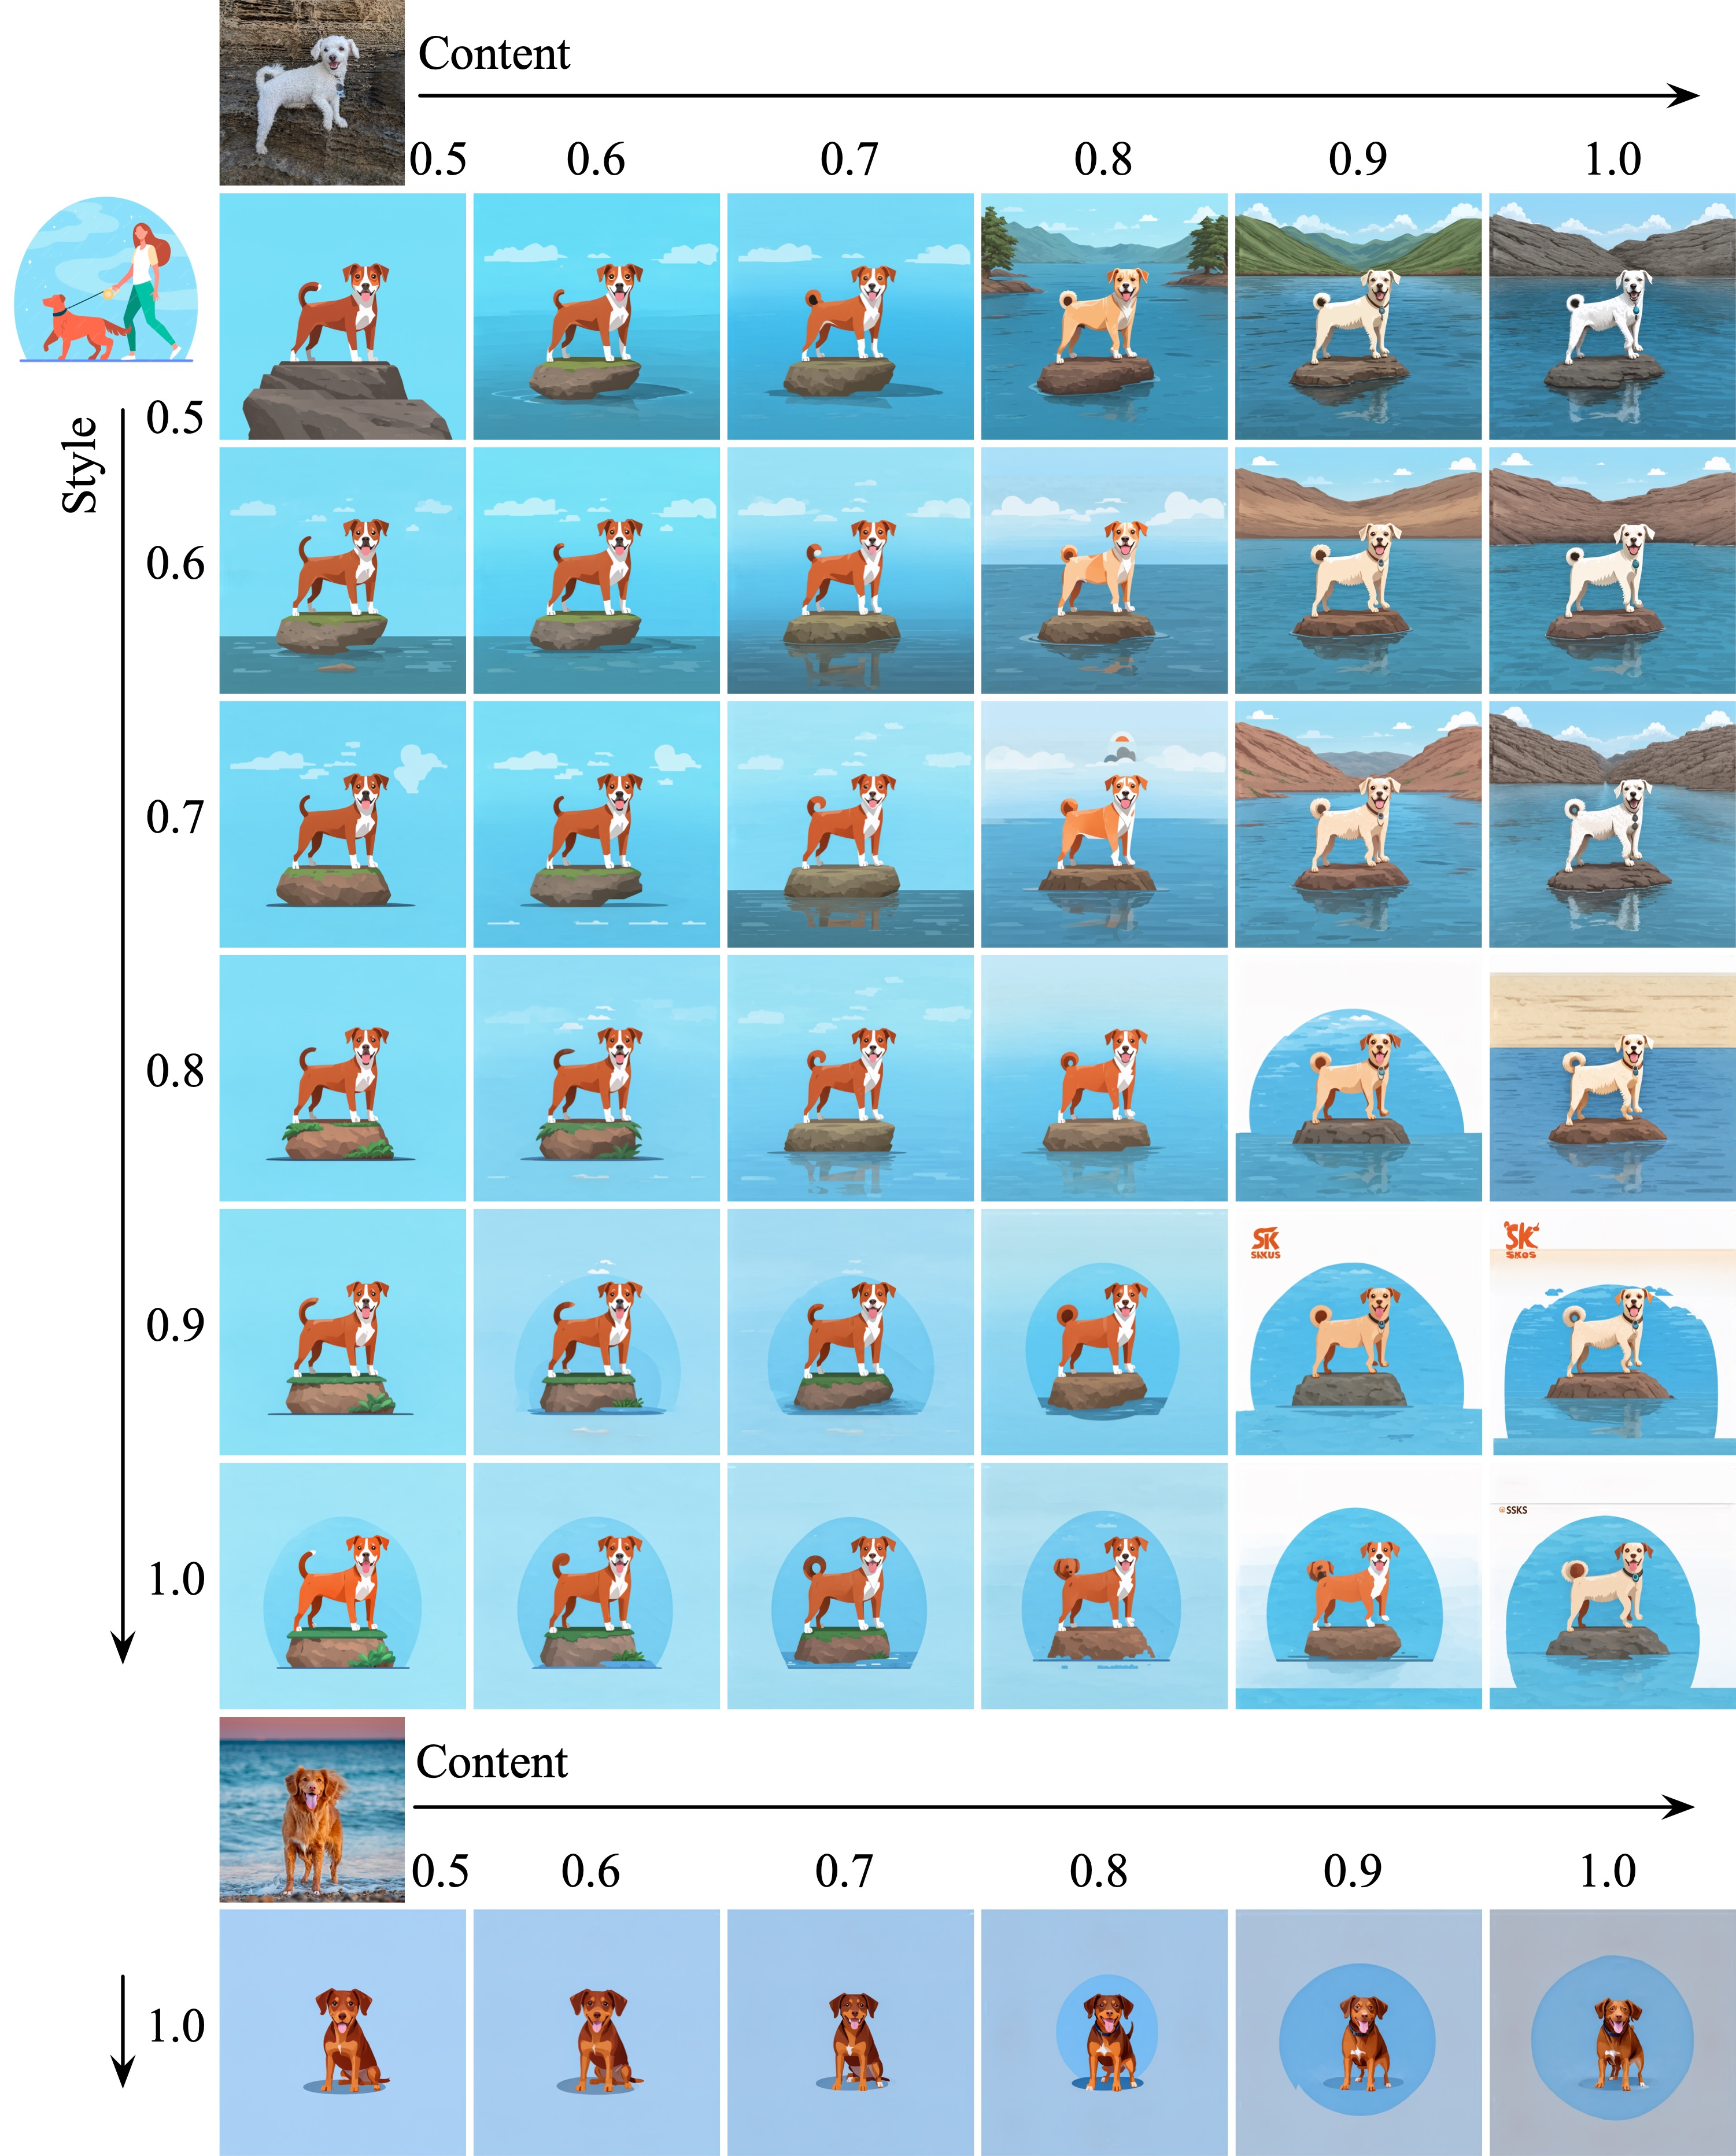}
    \caption{\textbf{Comprehensive ablation study on scaling coefficients for content-style fusion based on SD3.} We demonstrate the generation results under various combinations of content and style scaling coefficients. The experiments validate the flexibility and robustness of our approach in achieving fine-grained control over content-style fusion through different coefficient combinations. Please zoom in to view details.}
    \label{fig:appendix-ablation-coeff-sd3}
\end{figure*}

\begin{figure*}[th]
    \centering
    \includegraphics[width=\linewidth]{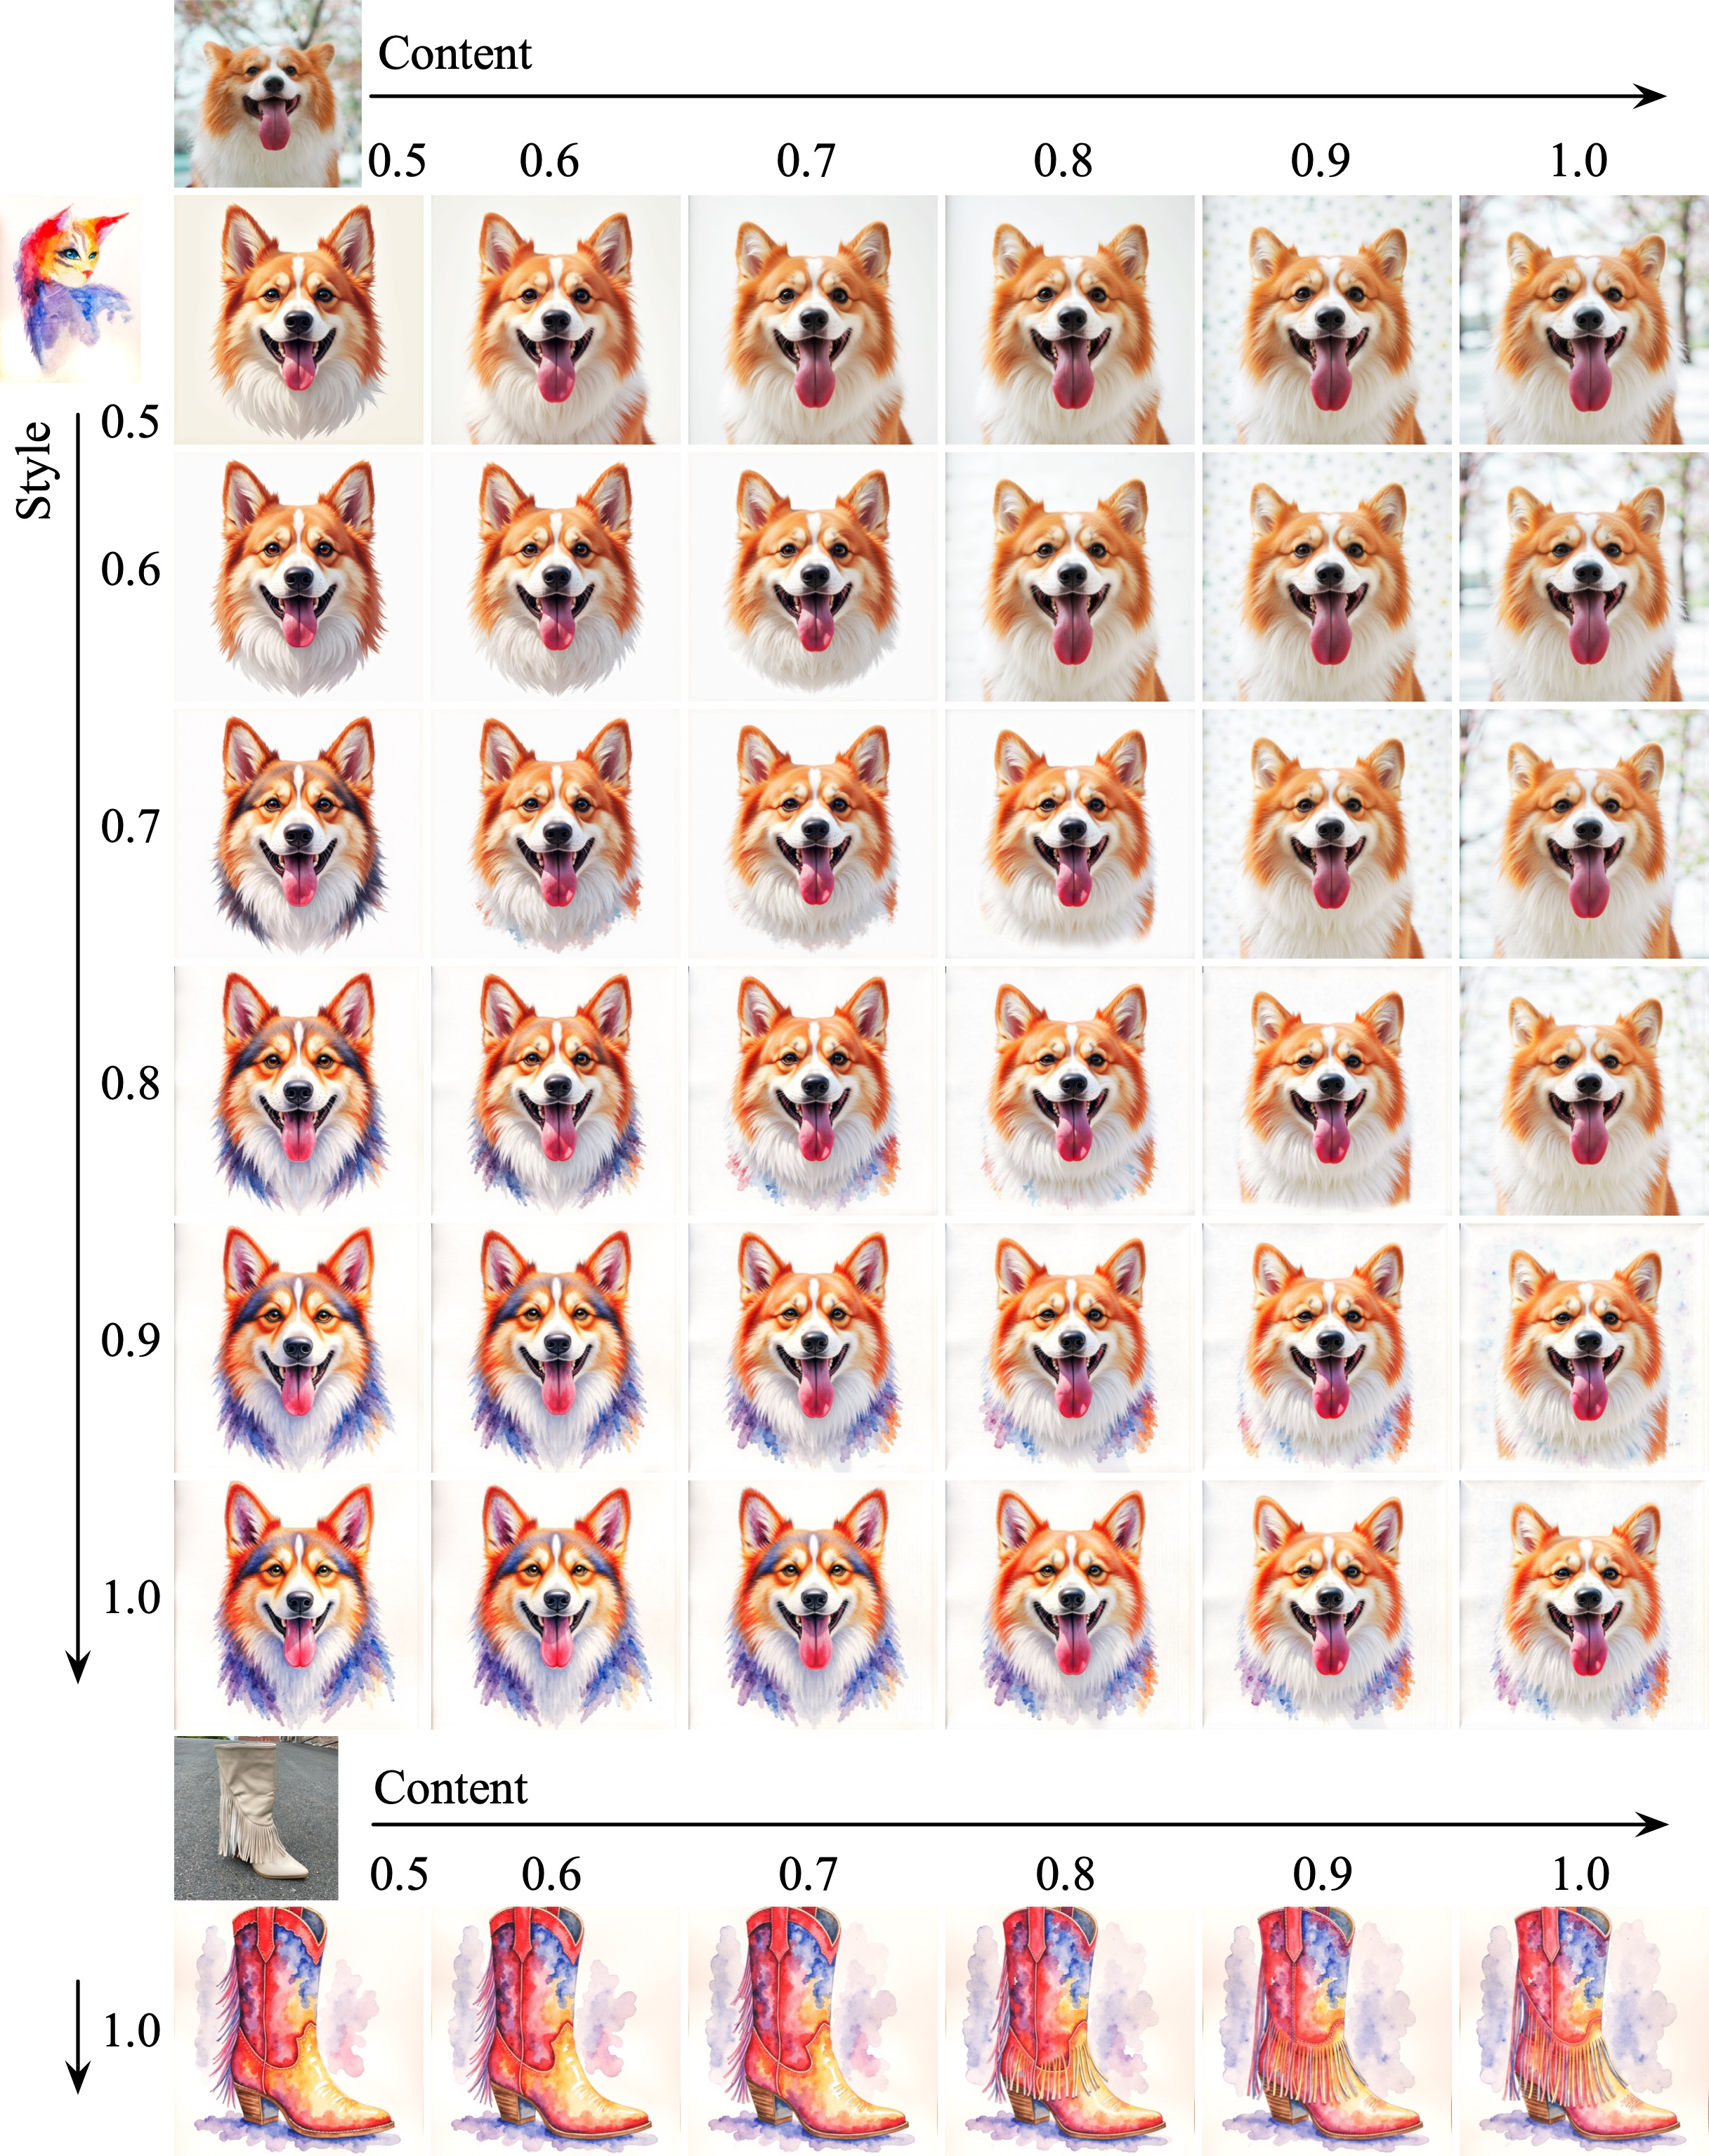}
    \caption{\textbf{Comprehensive ablation study on scaling coefficients for content-style fusion based on FLUX.1-dev.} The experiments validate the flexibility and robustness of our approach in achieving fine-grained control over content-style fusion through different coefficient combinations. Please zoom in to view details.}
    \label{fig:appendix-ablation-coeff-flux}
\end{figure*}

\subsection{User Study}
To evaluate the perceptual quality of our results, we conducted a comprehensive user study with 47 participants (40 males and 7 females). The participants represented a diverse demographic, with ages ranging from 22 to 45 years (mean age: 31.2). Among the participants, 15 were computer vision researchers, 12 were professional designers, and 20 were general users with basic knowledge of image editing. This diverse composition ensured a balanced evaluation from both technical and aesthetic perspectives.

Each participant was asked to rate the quality of generated images from different methods on a scale of 0-5, where 0 indicates poor quality and 5 indicates excellent quality. To facilitate the evaluation process, we designed an intuitive rating interface (shown in Figure~\ref{fig:screenshot_of_user_study}) that allows participants to easily assess and score the generated images. The evaluation criteria focused on both content preservation and style transfer aspects. The ratings reported in Table~\ref{tab:quantitative-results} represent the average scores given by participants for each method. The consistently higher ratings achieved by our method (4.07 for SDXL, 4.14 for SD3, and 3.96 for FLUX.1-dev) compared to baseline approaches demonstrate the superior perceptual quality across different backbone models.

\subsection{Additional Qualitative Results}

To comprehensively demonstrate the effectiveness and versatility of our QR-LoRA framework, we present extensive qualitative results across different backbone models and diverse application scenarios. First, we conduct a thorough comparative analysis through Figure~\ref{fig:appendix-comparison}, which showcases our method's superior performance against state-of-the-art approaches across SDXL, SD3, and FLUX.1-dev models. The results consistently demonstrate QR-LoRA's ability to achieve better content preservation while maintaining high-fidelity style transfer, regardless of the underlying model architecture.

\begin{figure*}[th]
    \centering
    \includegraphics[width=\linewidth]{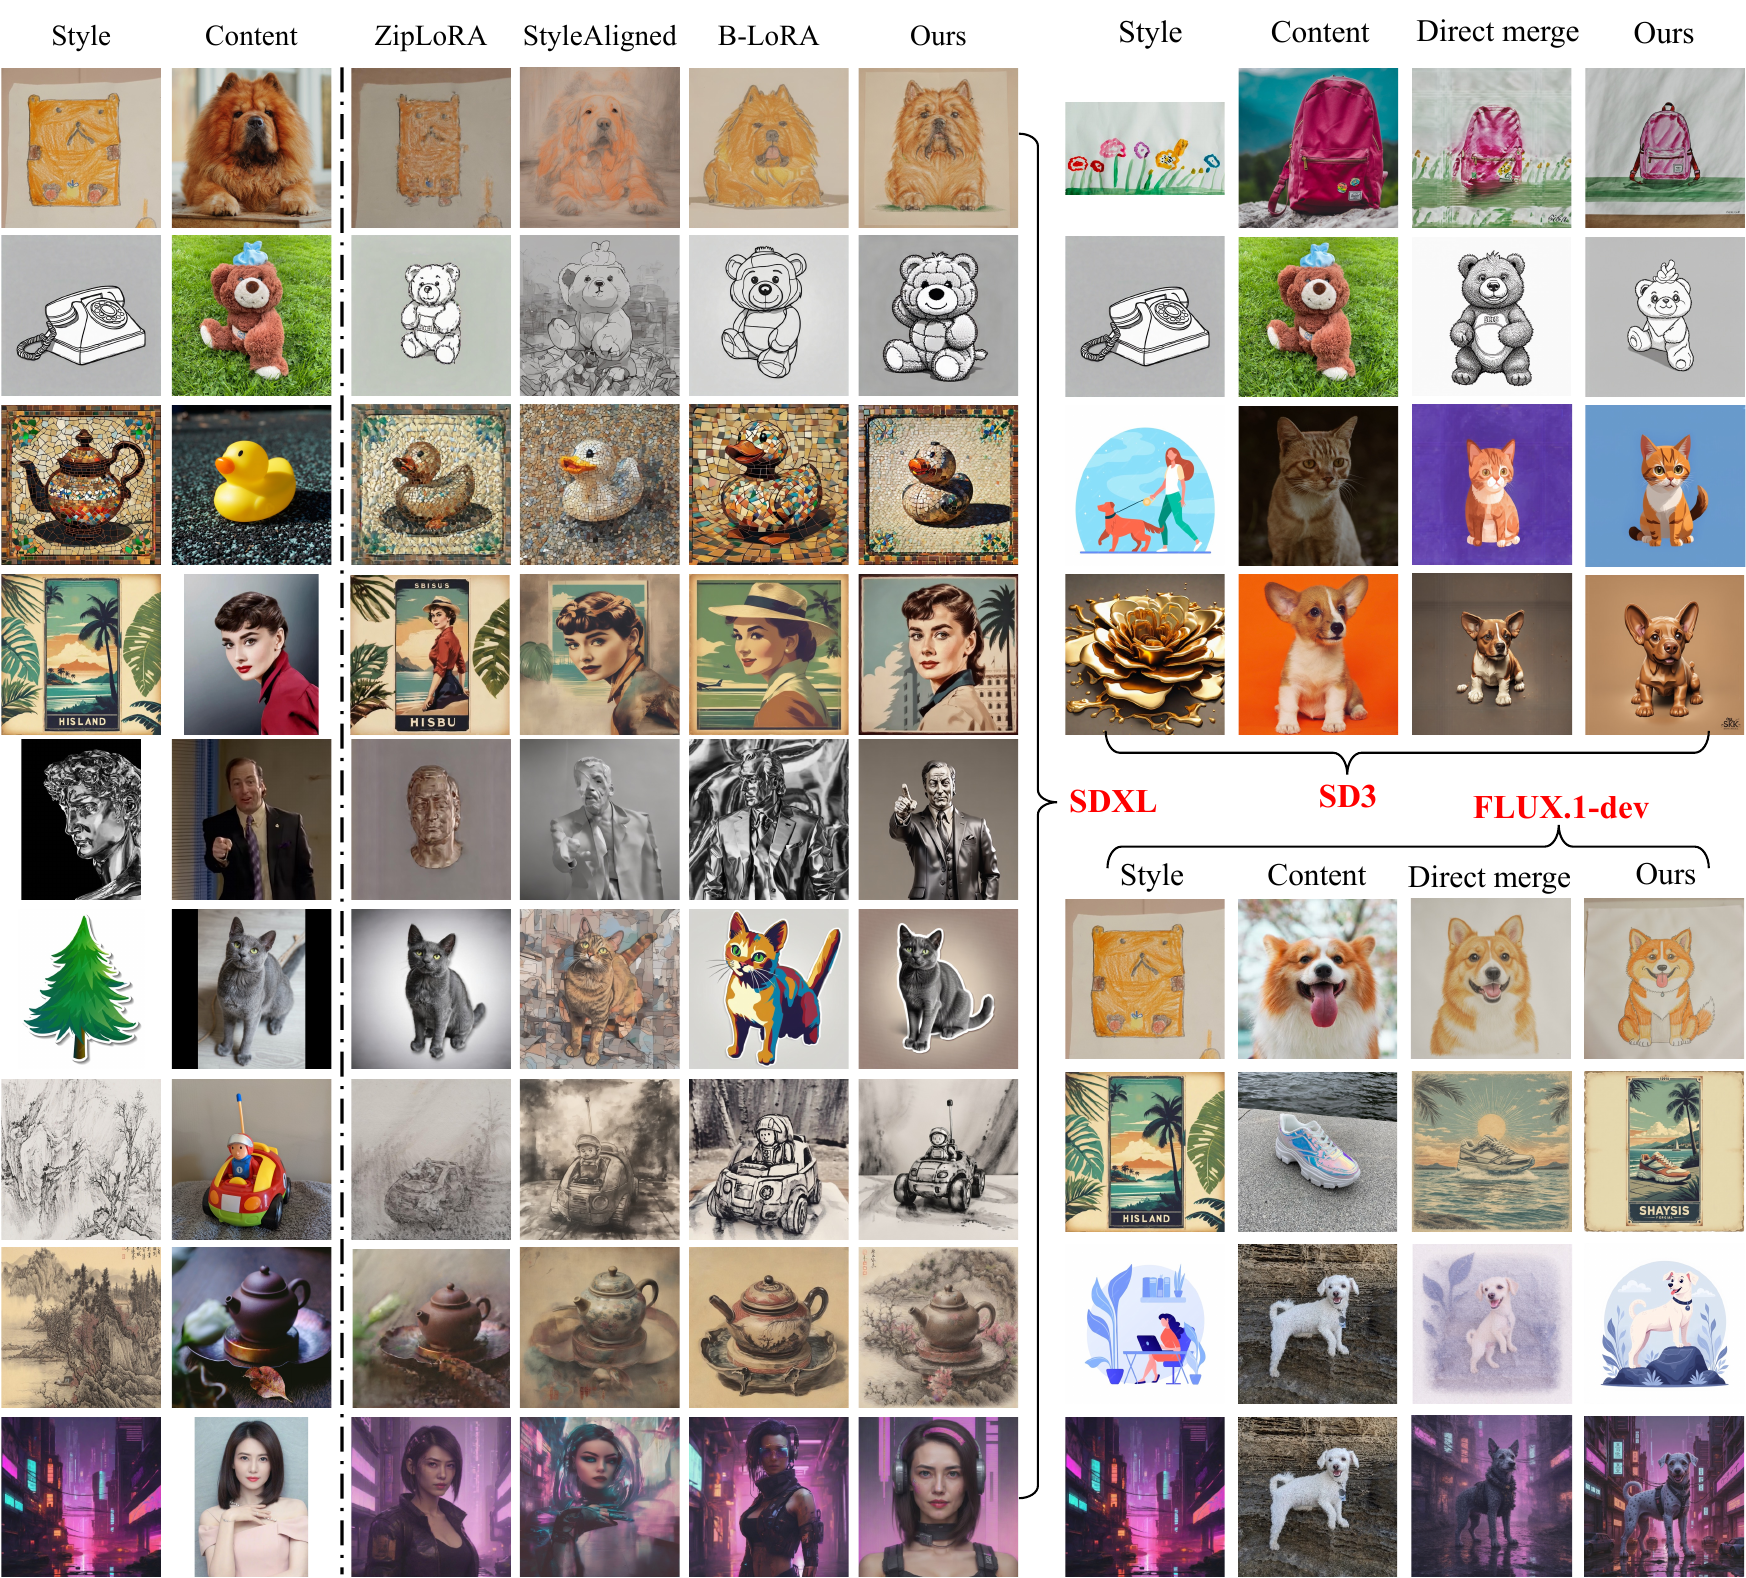}
    \caption{\textbf{Extended qualitative comparison results.} Comparison of QR-LoRA against state-of-the-art methods on SDXL, SD3, and FLUX.1-dev models, demonstrating consistent superior performance across different scenarios. Please zoom in to view details.}
    \label{fig:appendix-comparison}
\end{figure*}

To further validate the model-agnostic nature of our approach, we present a comprehensive set of generation results across different backbone architectures. Figures~\ref{fig:appendix-vis1}, \ref{fig:appendix-vis2}, and \ref{fig:appendix-vis3} showcase diverse generation results on SDXL, demonstrating our method's capability in handling various challenging scenarios while maintaining high visual quality and style fidelity. The results span a wide range of content types and artistic styles, from intricate architectural details to subtle texture variations.

\begin{figure*}[th]
    \centering
    \includegraphics[width=\linewidth]{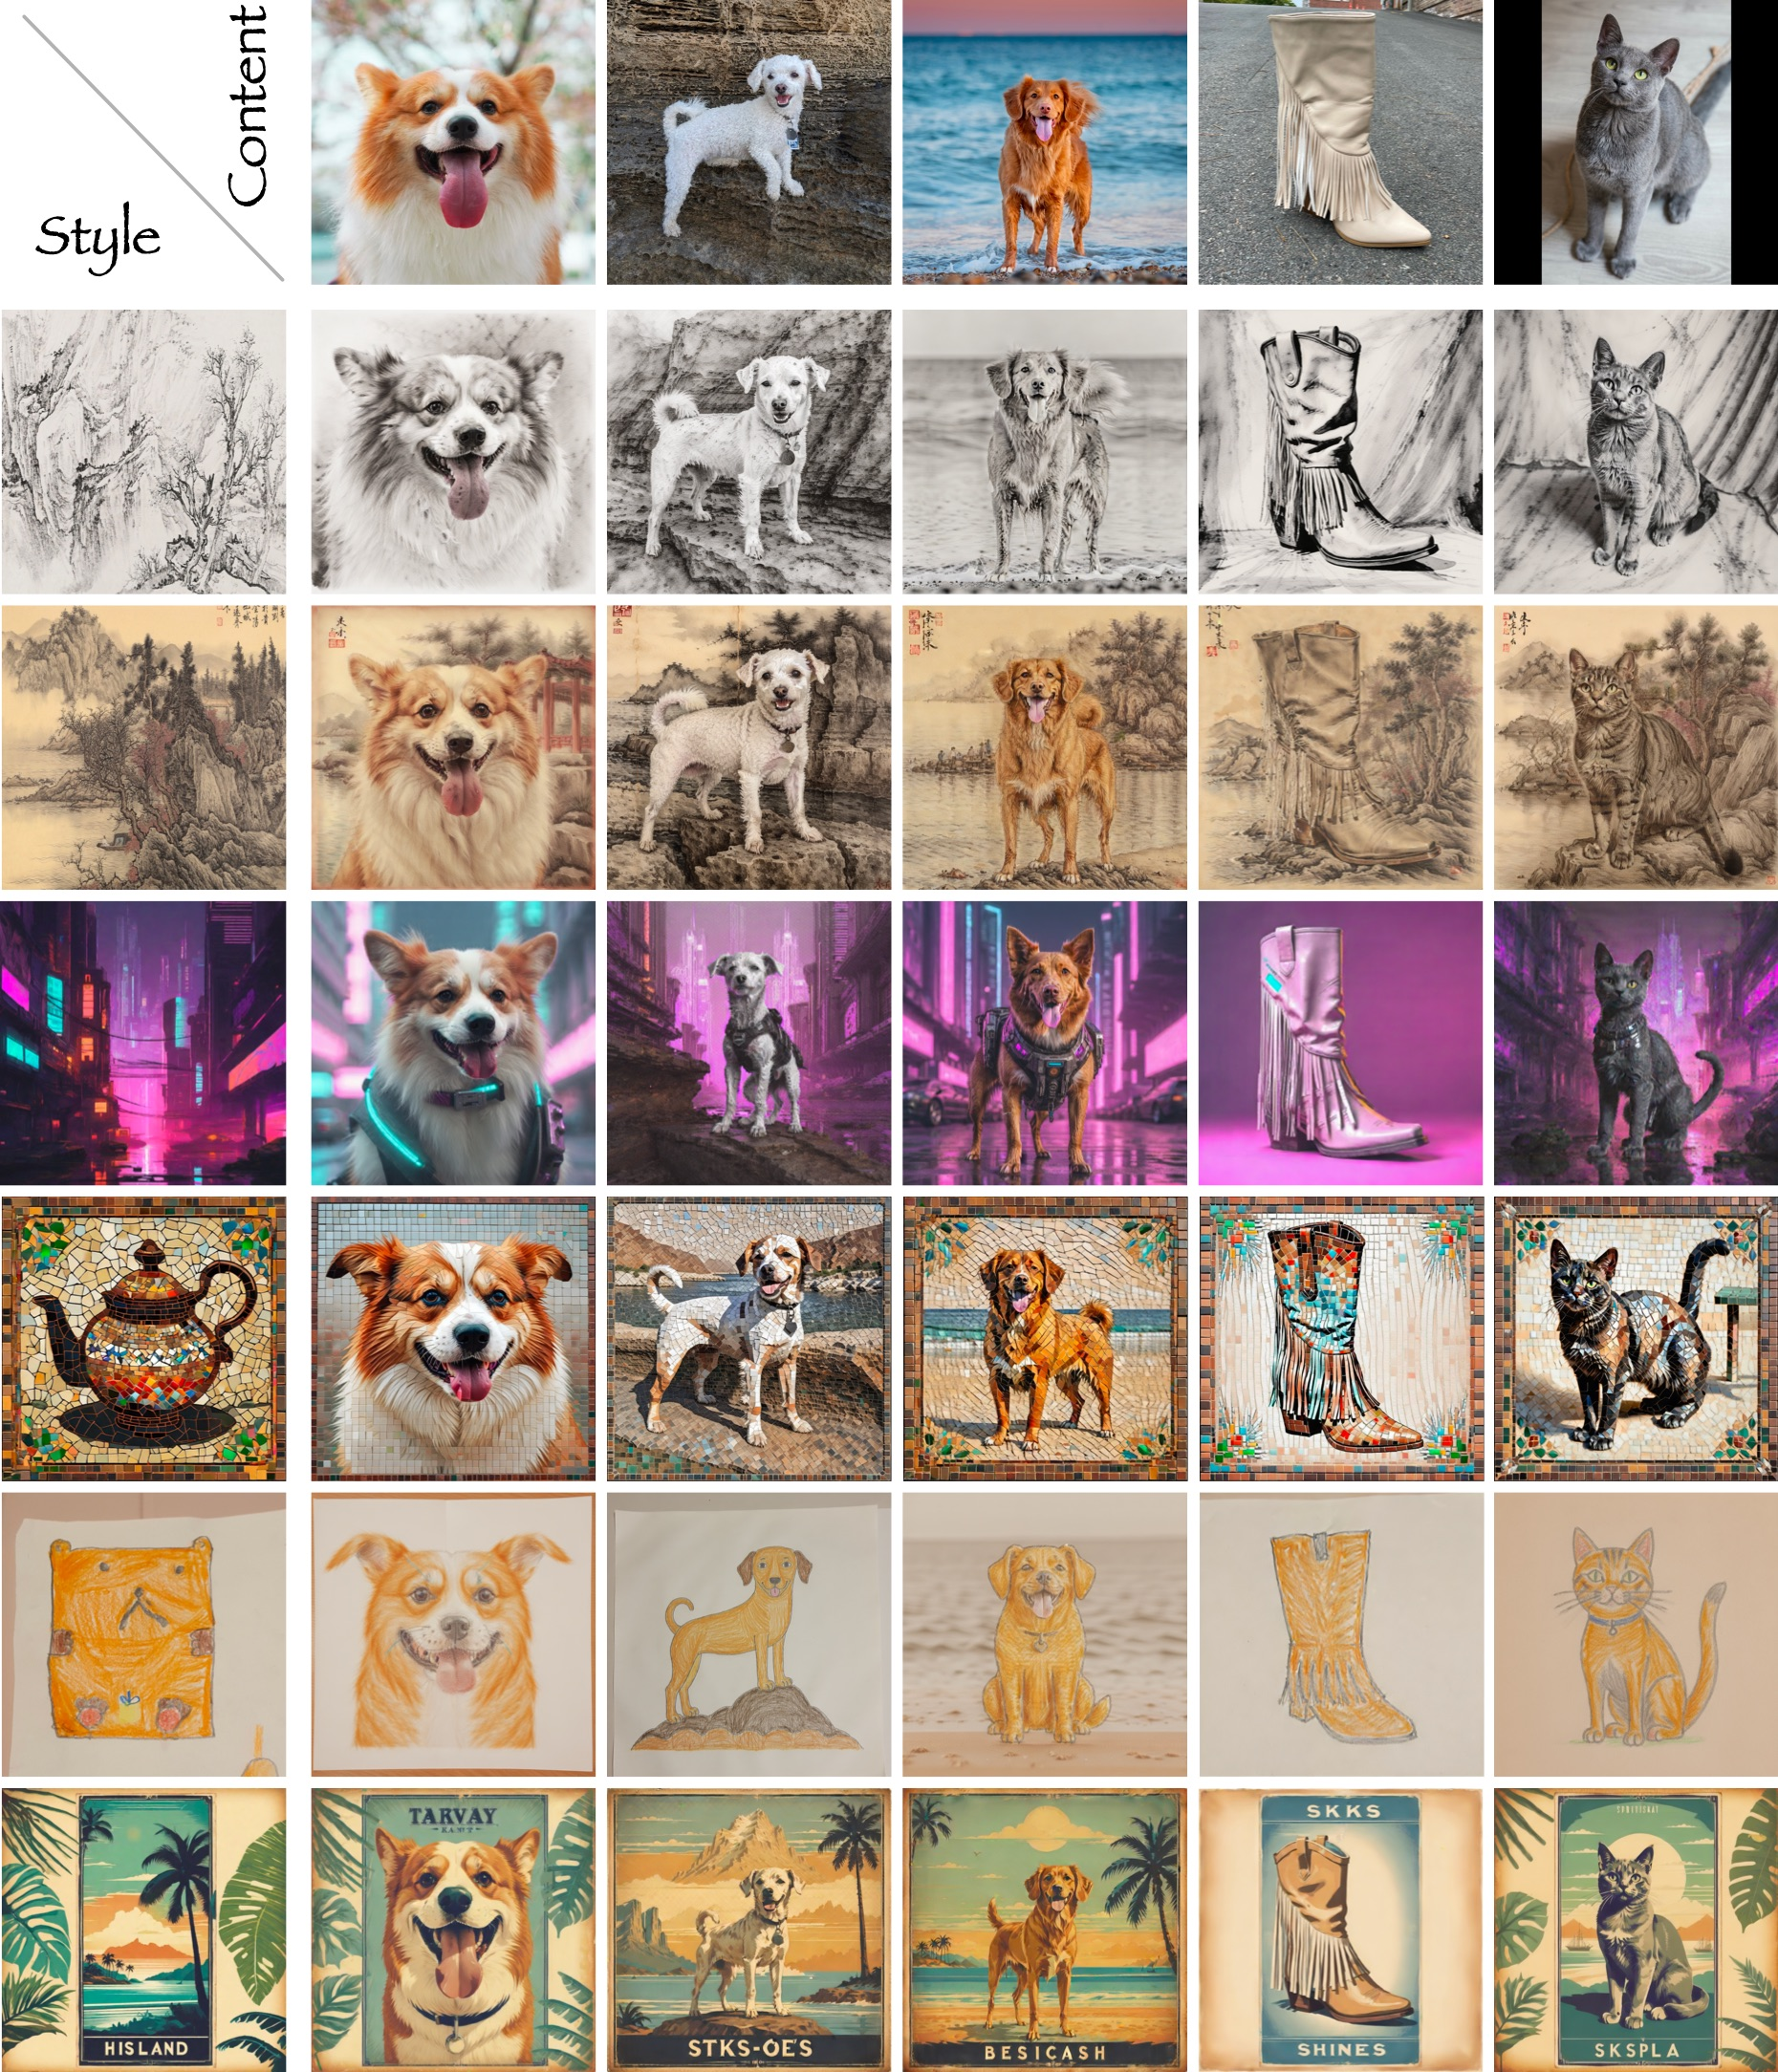}
    \caption{\textbf{Diverse generation results based on SDXL.} Additional examples showcasing QR-LoRA's capability in handling various style-content combinations. Our method successfully preserves intricate content details while effectively transferring diverse artistic styles, from painterly effects to digital art aesthetics. Please zoom in to view details.}
    \label{fig:appendix-vis1}
\end{figure*}

\begin{figure*}[th]
    \centering
    \includegraphics[width=\linewidth]{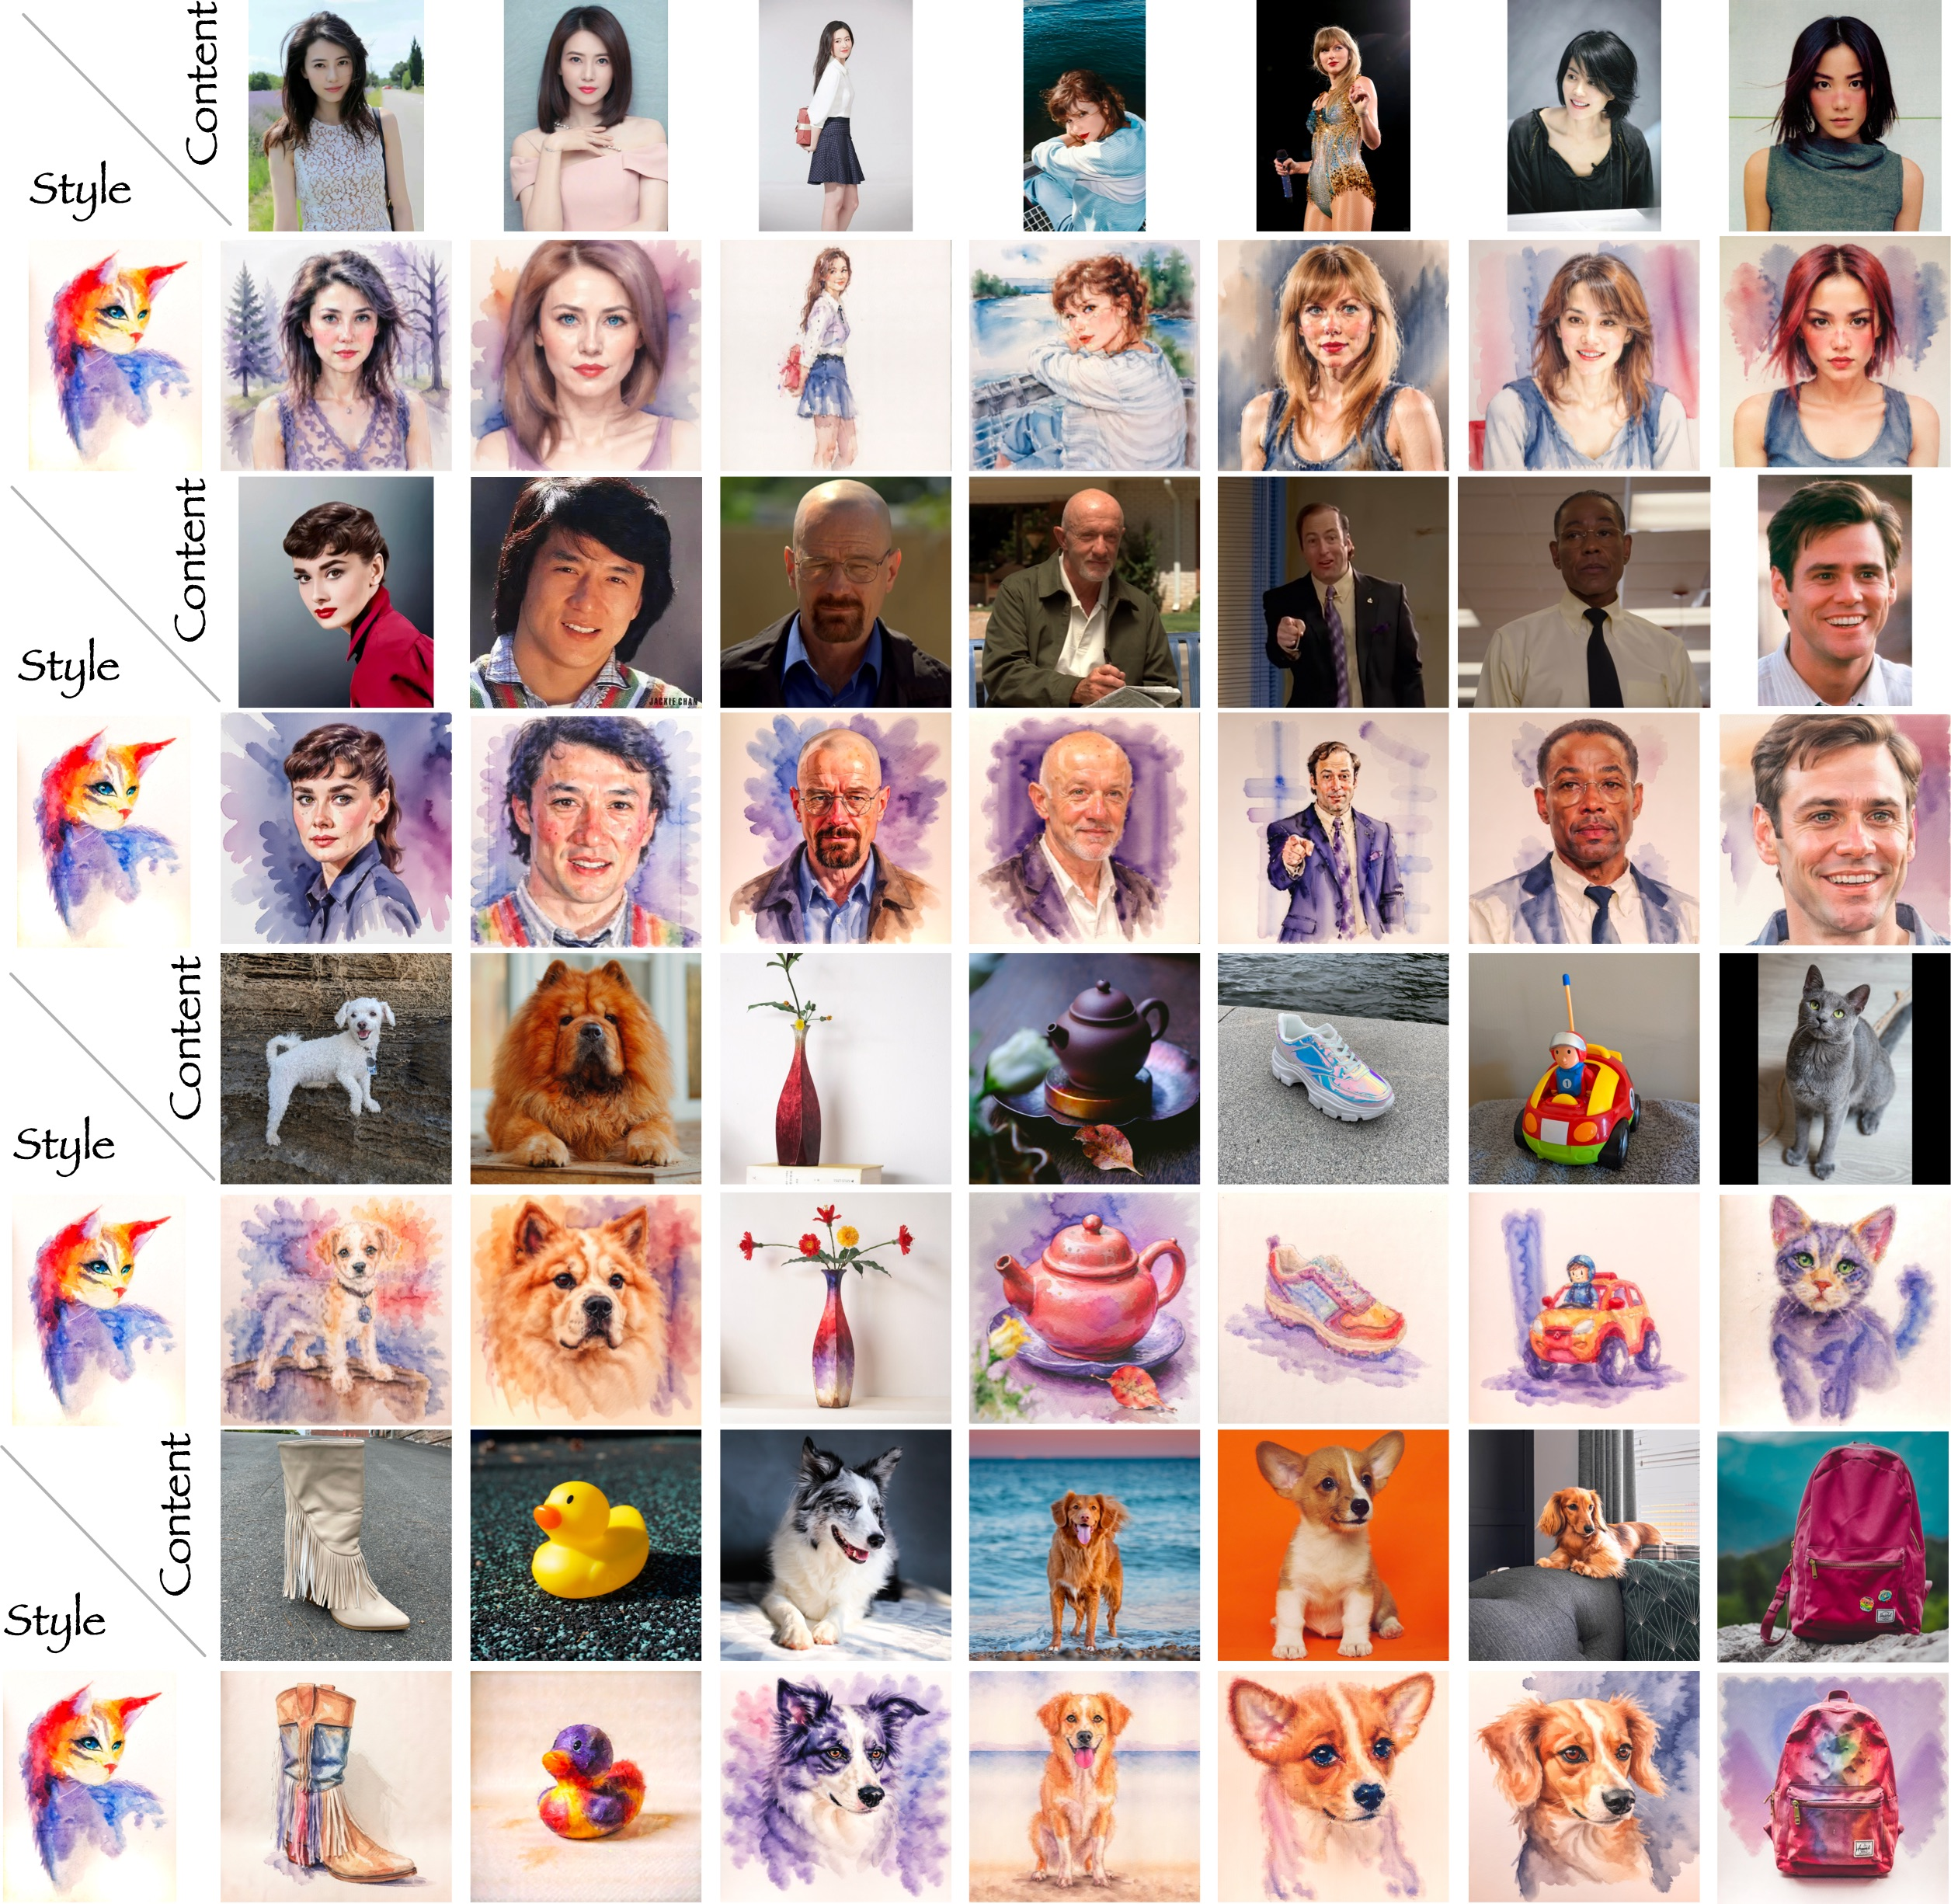}
    \caption{\textbf{Diverse generation results on SDXL.} Additional examples showcasing QR-LoRA's capability in handling various style-content combinations. Our method successfully preserves intricate content details while effectively transferring diverse artistic styles, from painterly effects to digital art aesthetics. Please zoom in to view details.}
    \label{fig:appendix-vis2}
\end{figure*}

\begin{figure*}[th]
    \centering
    \includegraphics[width=\linewidth]{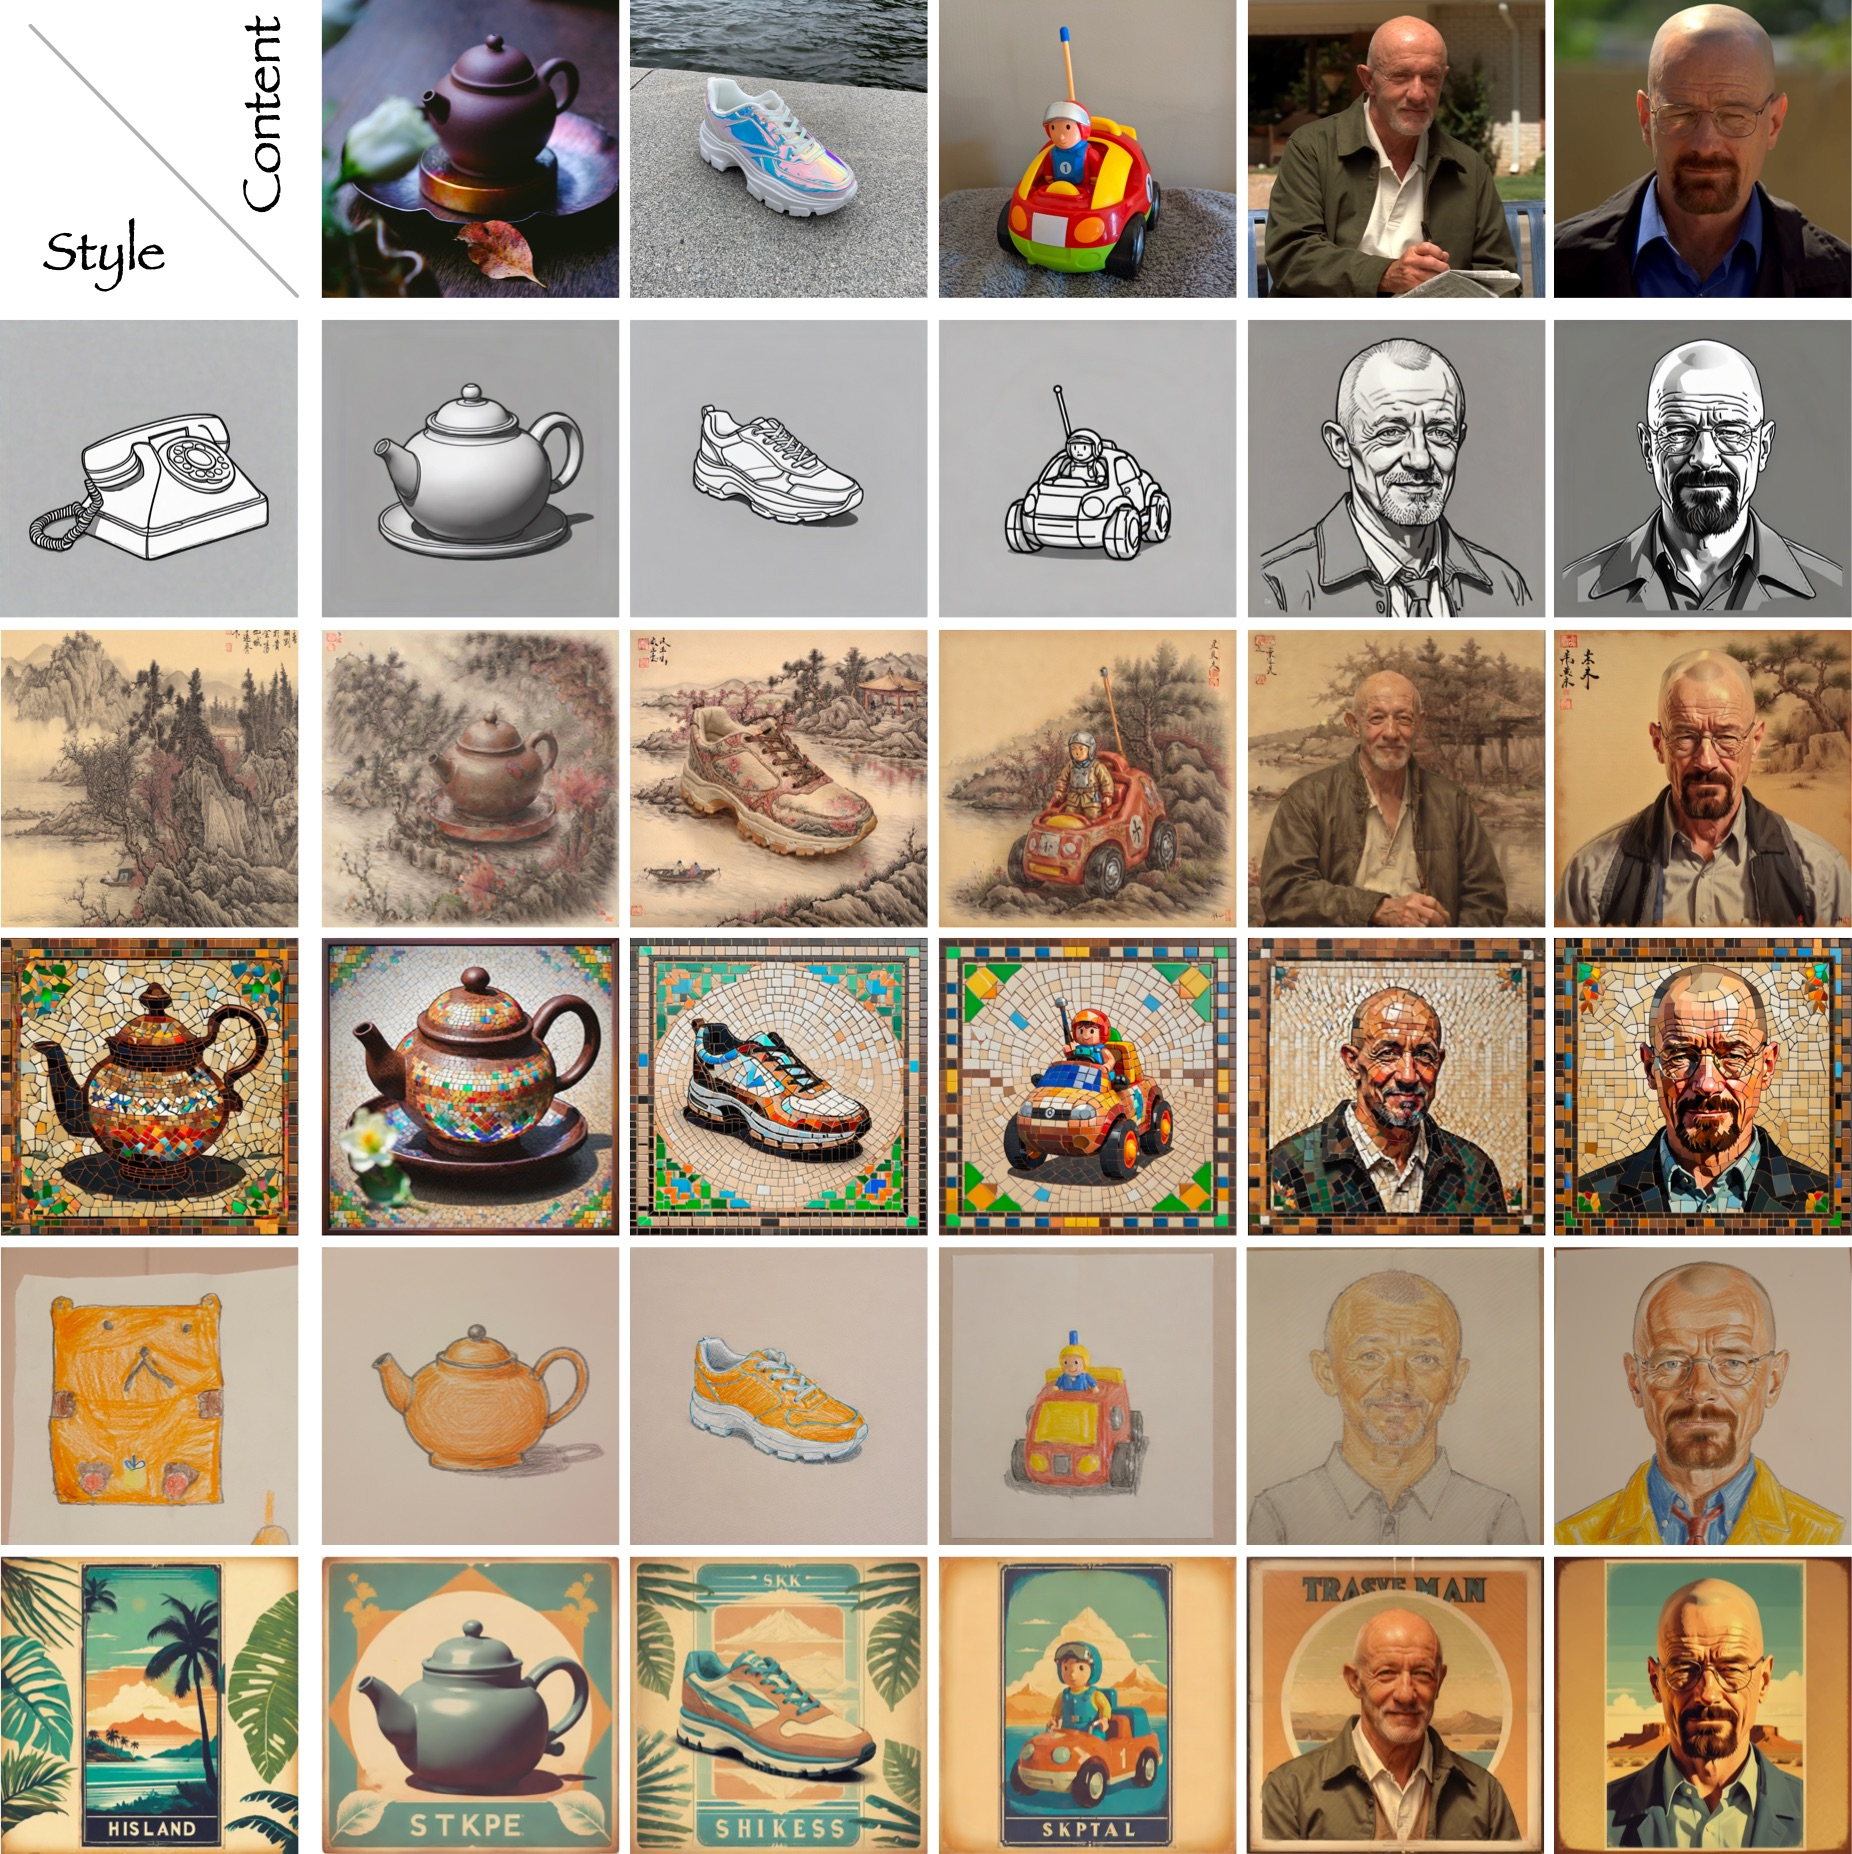}
    \caption{\textbf{Diverse generation results on SDXL.} Additional examples showcasing QR-LoRA's capability in handling various style-content combinations. Our method successfully preserves intricate content details while effectively transferring diverse artistic styles, from painterly effects to digital art aesthetics. Please zoom in to view details.}
    \label{fig:appendix-vis3}
\end{figure*}

Extending our analysis to other backbone architectures, Figure~\ref{fig:appendix-vis4} presents generation results on SD3, while Figure~\ref{fig:appendix-vis5} shows results using FLUX.1-dev as the backbone. These examples demonstrate that QR-LoRA maintains its effectiveness across different model architectures, consistently producing high-quality results that effectively balance content preservation and style transfer.

\begin{figure*}[th]
    \centering
    \includegraphics[width=\linewidth]{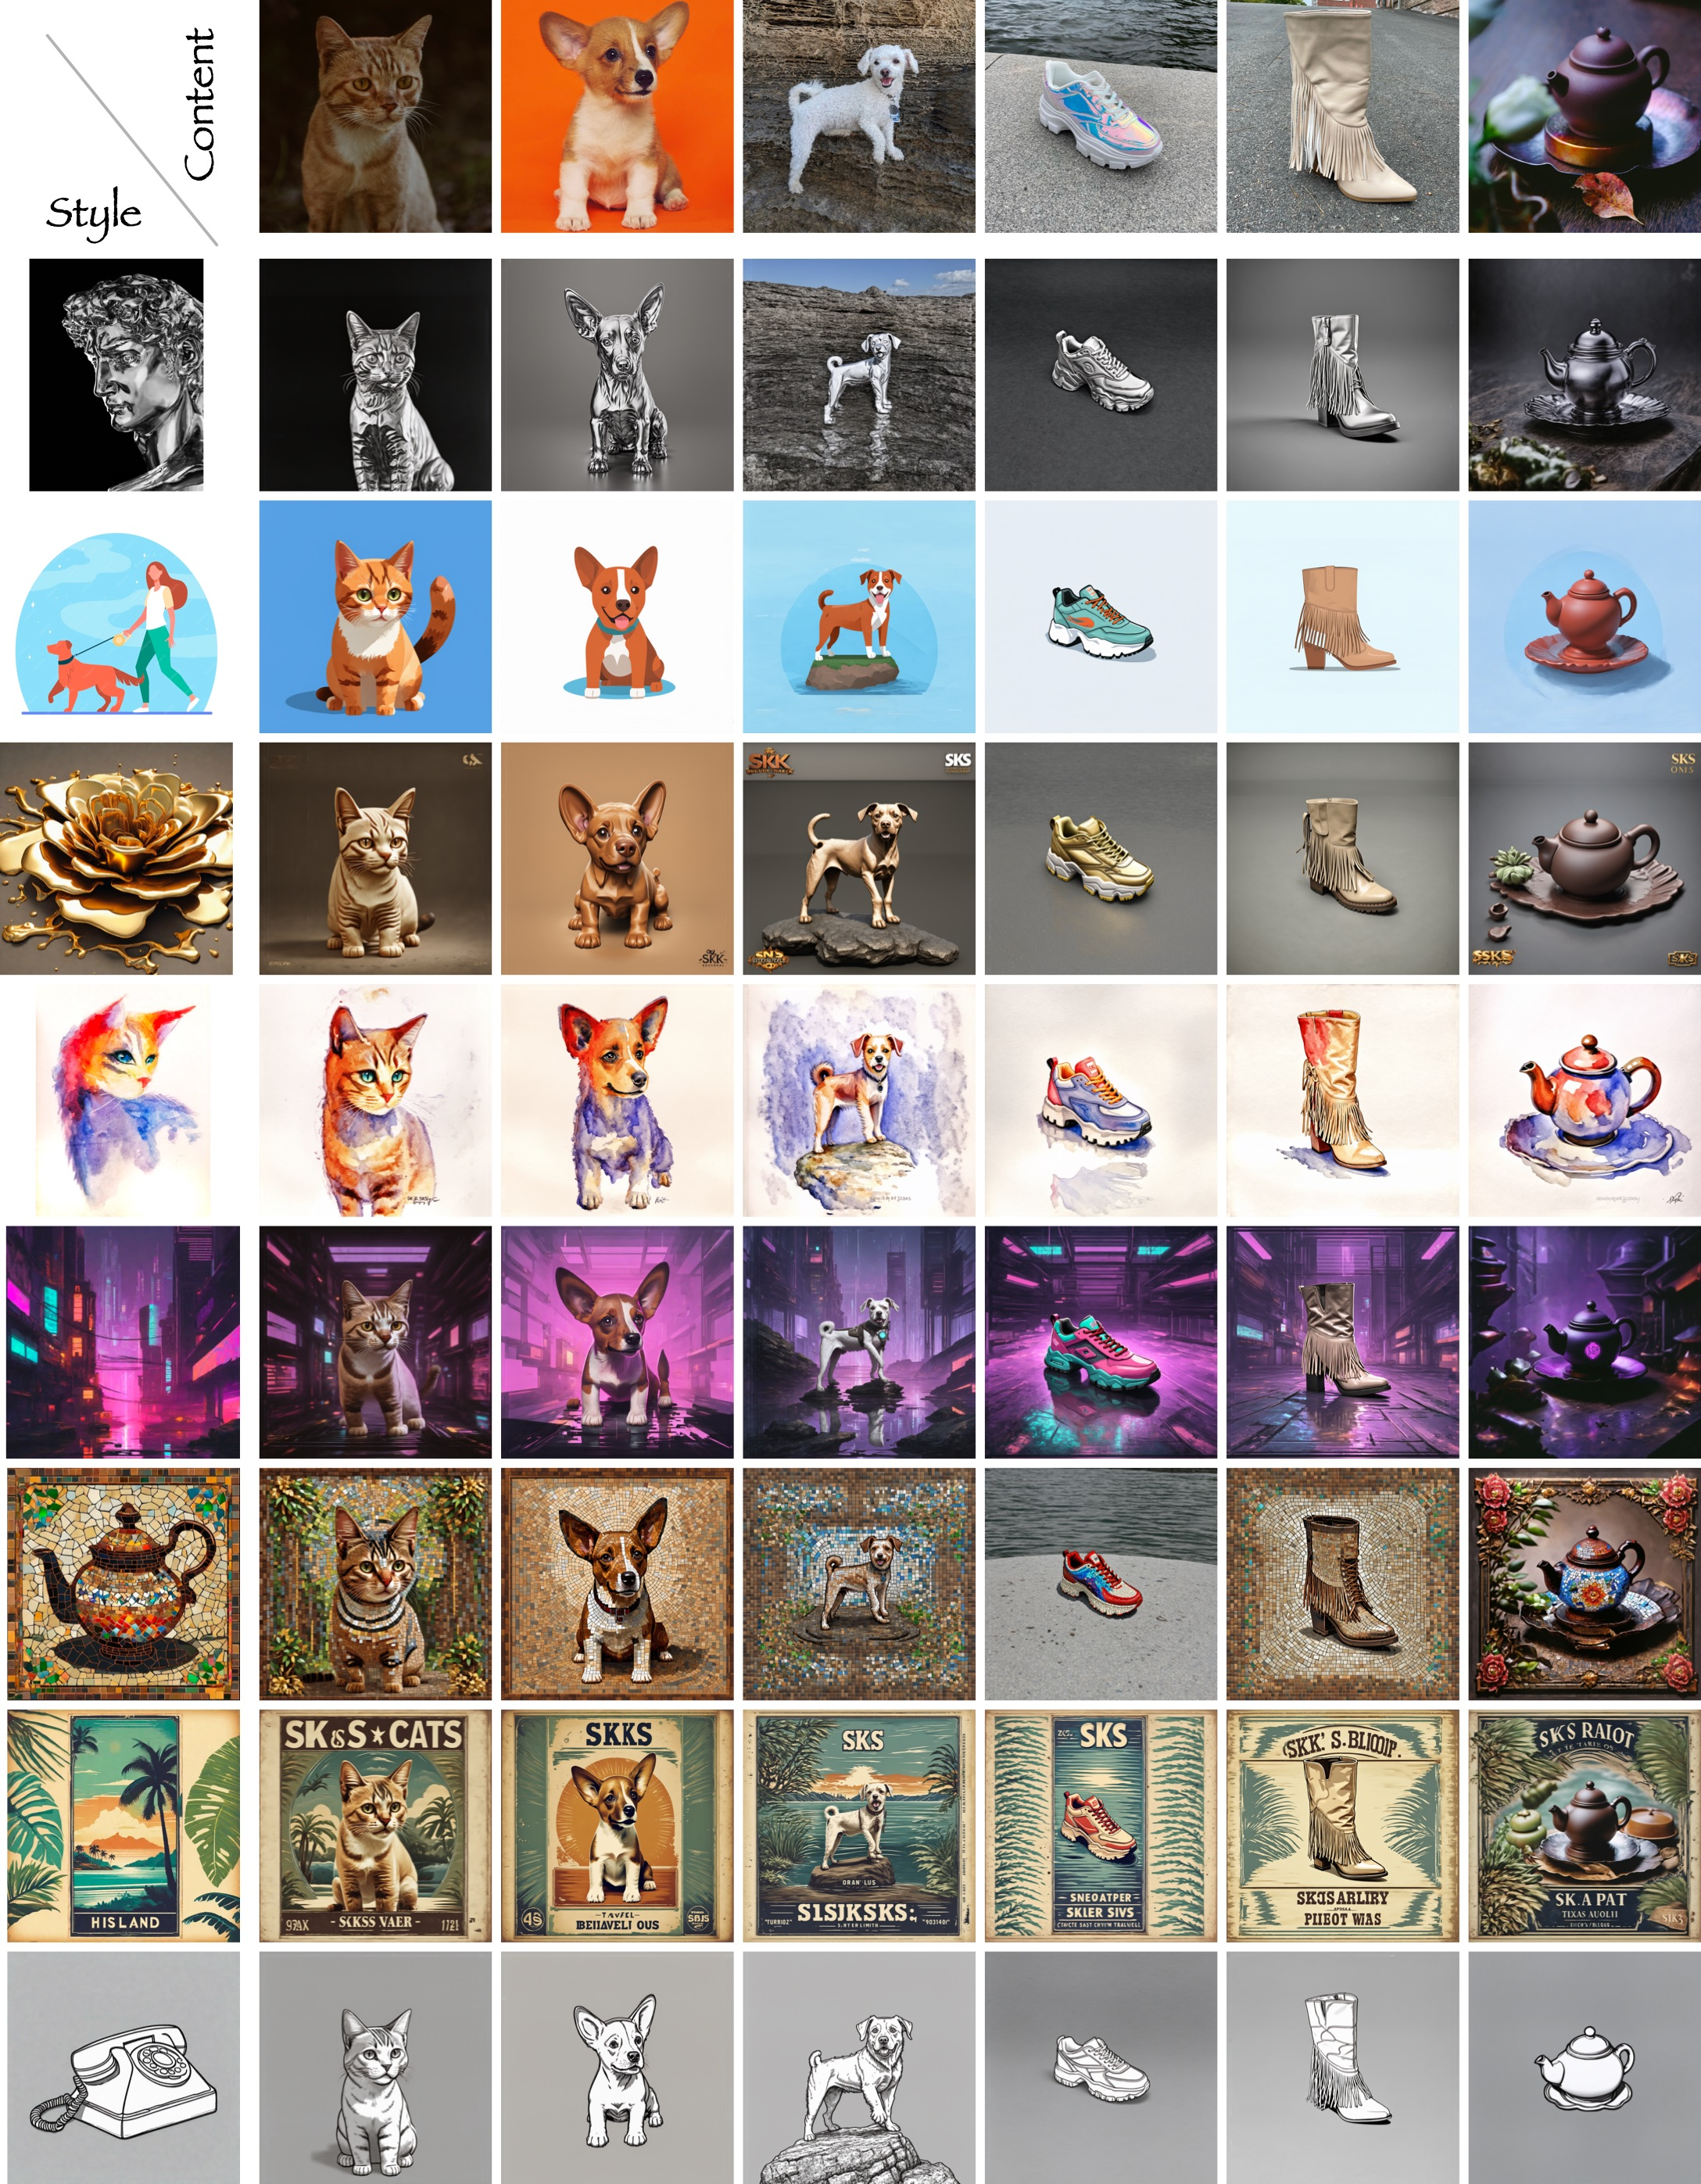}
    \caption{\textbf{Diverse generation results on SD3.} Additional examples showcasing QR-LoRA's capability in handling various style-content combinations.}
    \label{fig:appendix-vis4}
\end{figure*}

\begin{figure*}[th]
    \centering
    \includegraphics[width=\linewidth]{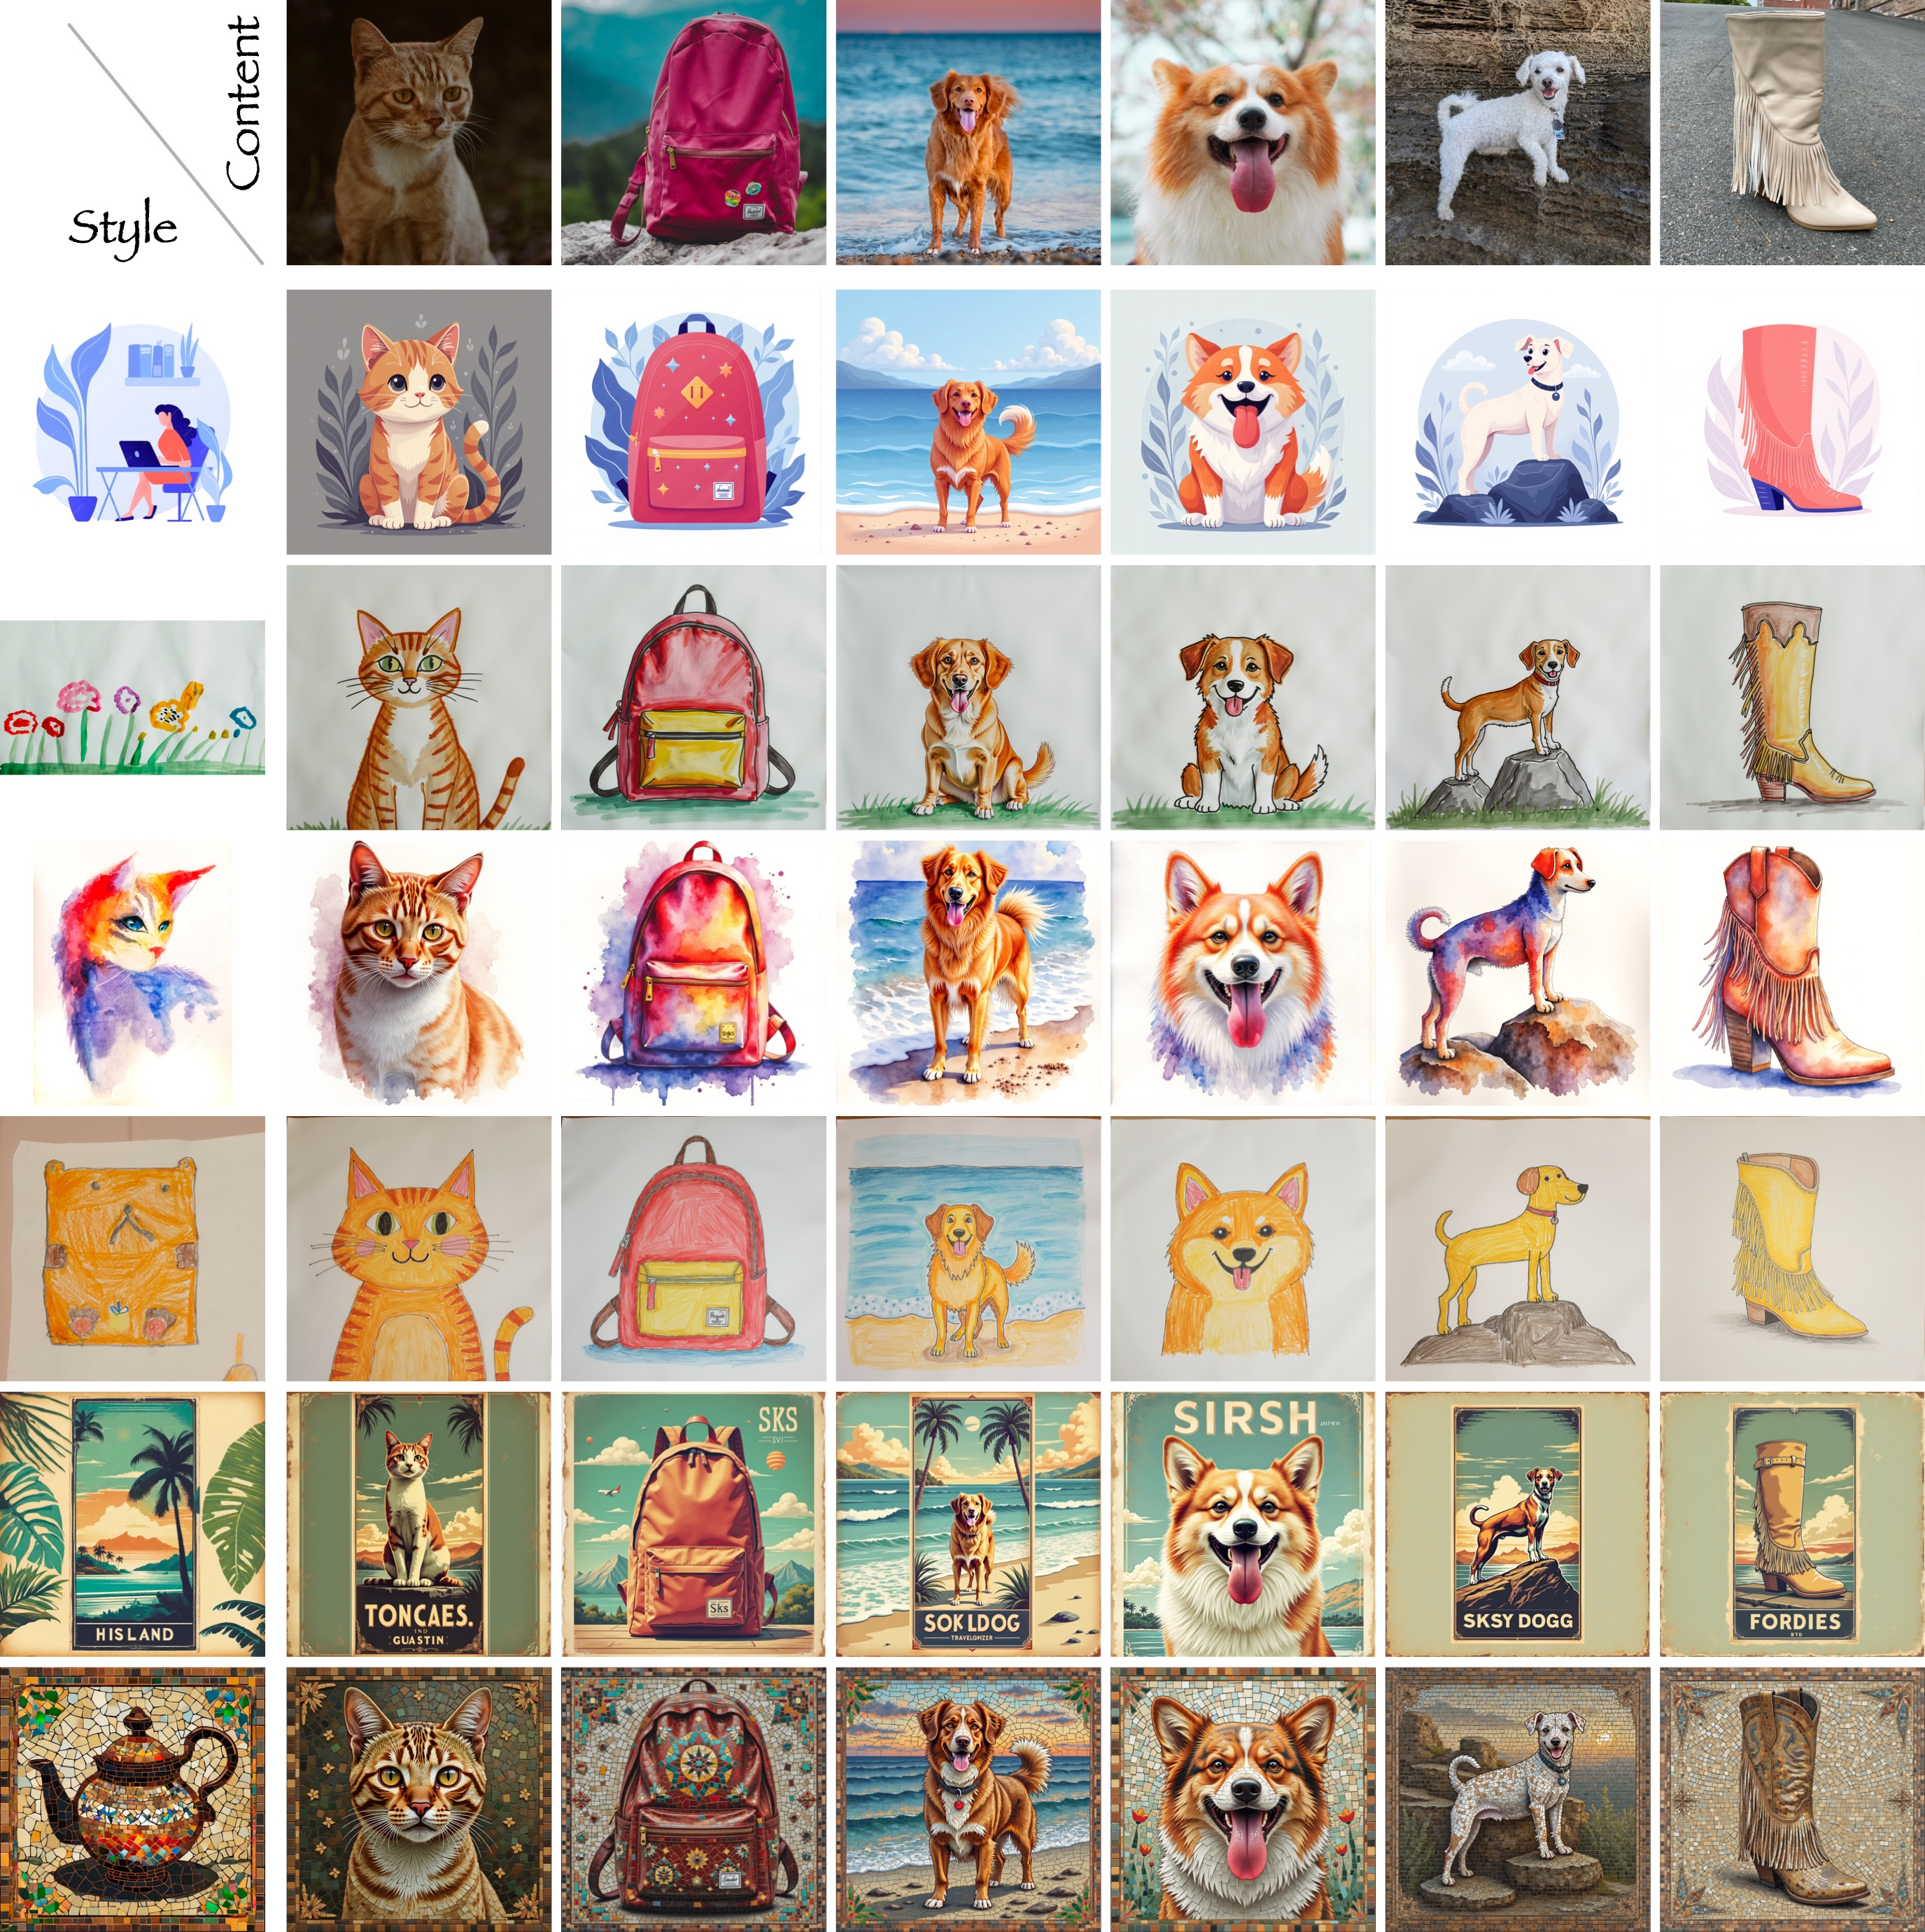}
    \caption{\textbf{Diverse generation results on FLUX.1-dev.} Additional examples showcasing QR-LoRA's capability in handling various style-content combinations. Our method successfully preserves intricate content details while effectively transferring diverse artistic styles, from painterly effects to digital art aesthetics. Please zoom in to view details.}
    \label{fig:appendix-vis5}
\end{figure*}

Collectively, these results validate the robustness and generalization capability of our approach across diverse scenarios. The consistent high-quality performance across different content types (\eg, portraits, objects) and artistic styles (\eg, watercolor, digital art) demonstrates QR-LoRA's effectiveness in handling complex geometric structures, fine-grained textures, and dramatic style variations. This comprehensive evaluation further supports the model-agnostic nature of our method and its potential for broad application in various image generation and style transfer tasks.

\subsection{Ability to Re-contextualize}
Our method not only excels at fusing content and style but also enables further customization through text prompts. While maintaining the high-quality integration of content and style elements, our approach supports flexible scene manipulation through additional textual instructions, as shown in Figure~\ref{fig:appendix-recontextualize}. For instance, given a content image of a dog and a specific artistic style, we can generate variations like "wearing a hat" or "riding a bicycle" while preserving the desired style characteristics. This re-contextualization capability is particularly valuable in practical artistic applications, as it allows artists to explore diverse creative possibilities while maintaining consistent stylistic elements across different scenarios.

\begin{figure*}[th]
    \centering
    \includegraphics[width=\linewidth]{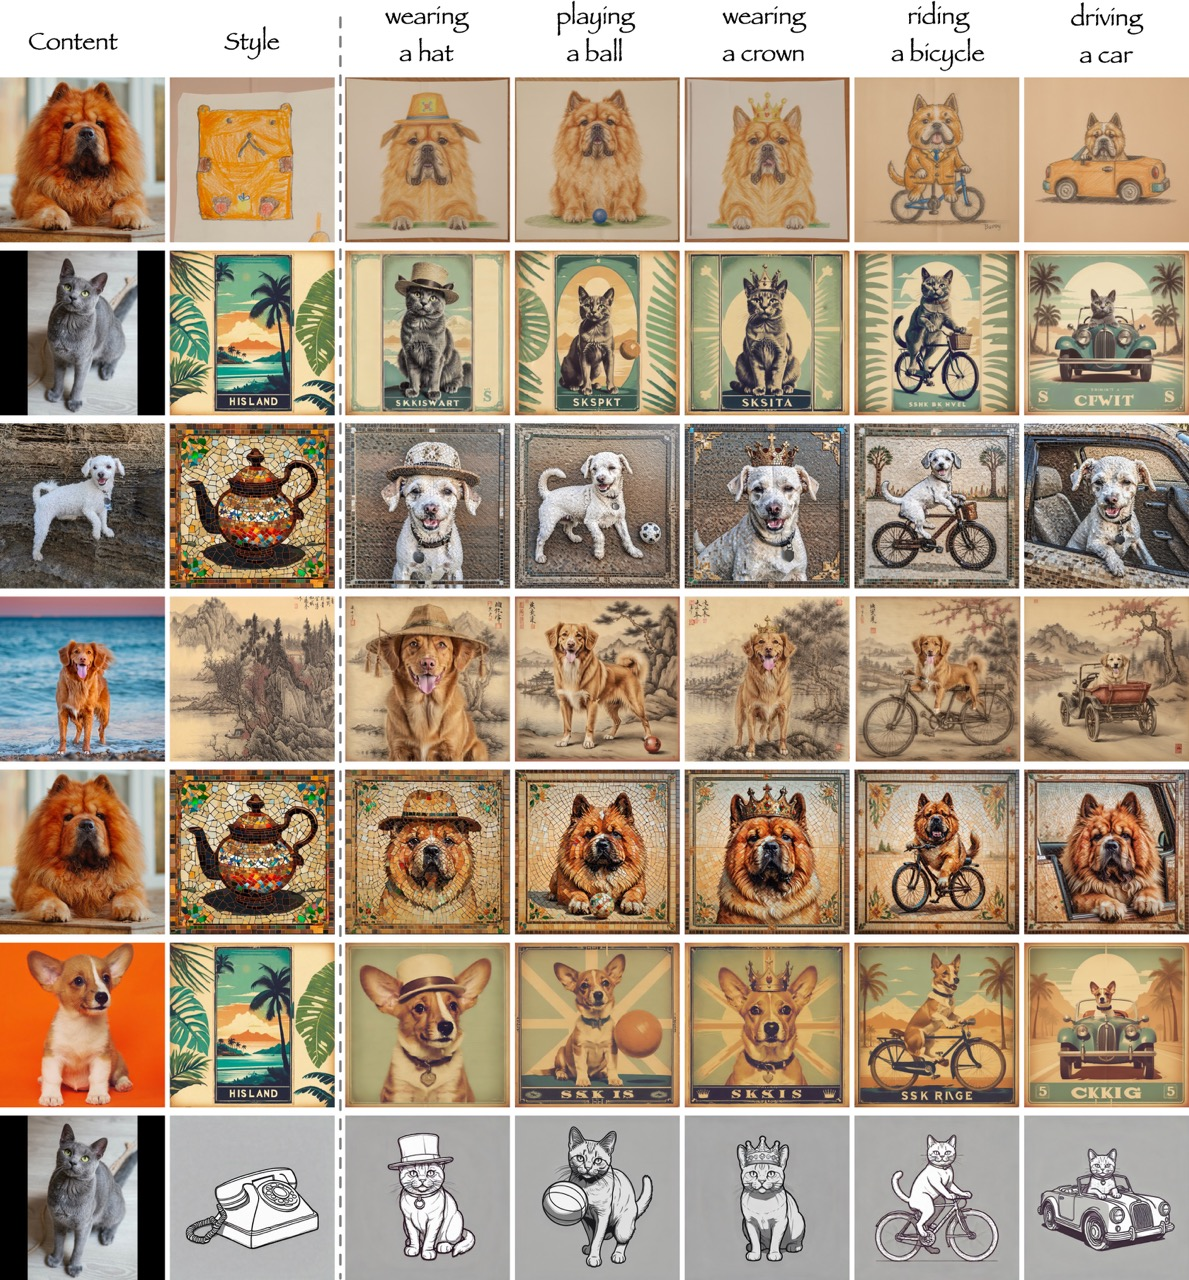}
    \caption{Demonstration of our method's re-contextualization capability. Given a content image and a style reference, our approach can generate variations through additional text prompts while maintaining style consistency. The examples show how different textual instructions (\eg., "wearing a hat", "riding a bicycle") guide the generation process to create diverse scenarios while preserving the original style characteristics.}
    \label{fig:appendix-recontextualize}
\end{figure*}

\subsection{The End}
We anticipate that our model-agnostic, low-rank efficient fine-tuning approach will provide a versatile solution for fusion tasks requiring robust disentanglement properties, such as the fusion of arbitrary style and content. This stands in contrast to the field's ongoing trend of pursuing specific disentanglement properties within particular models.
